# Supplementary material for: AiSciVision: A Framework for Specializing Large Multimodal Models in Scientific Image Classification
Source: arXiv:2410.21480 source file (2024-10-28)
Supplement: Supplementary file 1 [file aqua_example.pdf]

True Class: 1, LMM Prediction: 1 (Probability: 0.80), Supervised Prediction: 0 (Probability: 25.91)

### System:

You are an expert in satellite imagery analysis specializing in aquaculture pond detection. Your task is to determine whether a satellite image contains aquaculture ponds or not. Aquaculture ponds in satellite imagery typically appear as regular, geometric shapes with distinct water surfaces. They are often arranged in clusters or grids in coastal areas or inland water bodies. Key characteristics to look for include: 1. Geometric Patterns: Aquaculture ponds are usually rectangular or square in shape, forming distinct geometric patterns. 2. Water Color: The water in aquaculture ponds often has a different color or tone compared to natural water bodies, due to the high density of organisms and potential algae growth. 3. Surrounding Features: Look for access roads, feeding platforms, or other infrastructure associated with aquaculture operations. 4. Location: Aquaculture ponds are commonly found in coastal areas, estuaries, or near rivers and lakes. 5. Size and Scale: The size of aquaculture ponds can vary, but they are typically uniform within a single farm and arranged in an organized manner. 6. Texture: The water surface of aquaculture ponds often appears smoother than natural water bodies. Use your knowledge and the tools provided to make an accurate classification of whether aquaculture ponds are present in the given satellite image.

### User:

This is an example of a satellite image with an aquaculture pond. Describe what you see, noting the characteristics that identify it as an aquaculture pond.

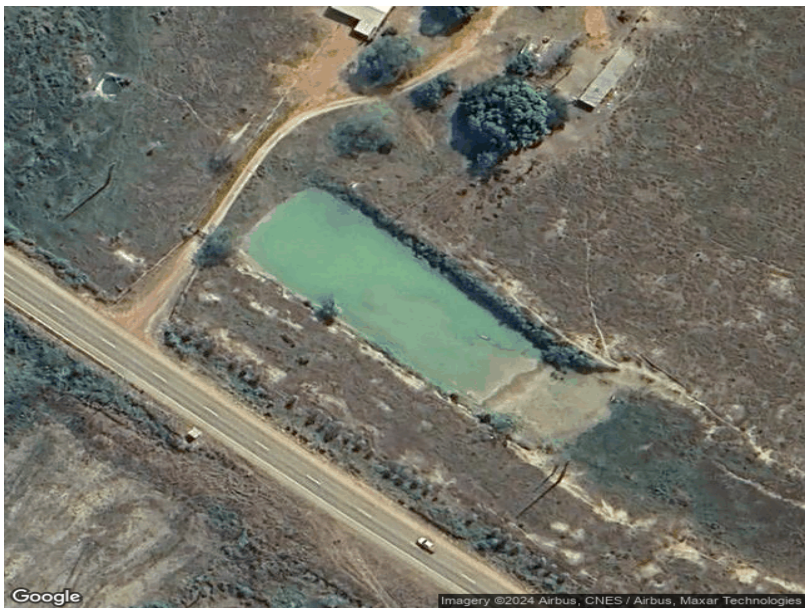

### Assistant:

In the provided satellite image, several characteristics identify the presence of an aquaculture pond:

**Geometric Pattern:** The pond is rectangular in shape, which is a common characteristic of aquaculture ponds. The straight edges and right angles suggest human-made construction.

**Water Color:** The water in the pond has a distinct greenish hue, which is different from the surrounding natural landscape. This color difference can be due to the high density of organisms or algae growth typical in aquaculture ponds.

**Surrounding Features:** There are access roads leading to the pond, indicating human activity and maintenance. Additionally, there are structures nearby that could be related to the aquaculture operation, such as storage or feeding facilities.

**Location:** The pond is situated in a relatively open area, which is typical for aquaculture ponds to allow easy access and management.

**Size and Scale:** The pond is uniform in size and appears to be part of a managed system, which is consistent with the organized nature of aquaculture farms.

**Texture:** The water surface appears relatively smooth compared to natural water bodies, indicating controlled conditions typical of aquaculture ponds.

These characteristics collectively suggest that the rectangular water body in the image is an aquaculture pond.

User:

This is an example of a satellite image without an aquaculture pond. Describe what you see, noting the absence of aquaculture ponds and any other relevant features.

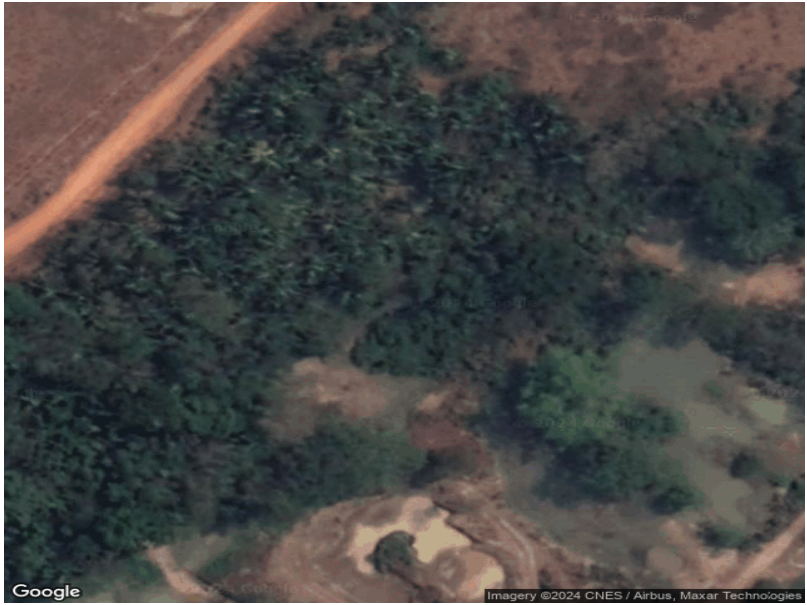

Assistant:

In the provided satellite image, there are no visible aquaculture ponds. Here are the observations and relevant features:

**Absence of Geometric Patterns:** There are no rectangular or square water bodies that would indicate the presence of aquaculture ponds. The area appears more natural and irregular in shape.

**Vegetation:** The image shows a dense area of vegetation, likely a forest or a plantation. The green canopy covers a significant portion of the image, indicating a natural or agricultural landscape rather than an aquaculture setup.

**Natural Water Bodies:** There are some patches of water visible, but they are irregular in shape and blend into the natural landscape. These do not exhibit the distinct, controlled appearance of aquaculture ponds.

**Surrounding Features:** There is a dirt road visible in the upper left corner of the image, but there are no signs of infrastructure typically associated with aquaculture operations, such as feeding platforms or storage facilities.

**Location and Land Use:** The area appears to be more rural and natural, with no clear signs of organized aquaculture activities. The land use seems to be more aligned with forestry or agriculture.

**Texture and Water Surface:** The water surfaces visible in the image do not have the smooth, controlled texture typical of aquaculture ponds. They appear more natural and varied.

Overall, the absence of geometric water bodies, the presence of dense vegetation, and the lack of aquaculture-related infrastructure indicate that this image does not contain aquaculture ponds.

User:

Here is the satellite image we need to classify as having an aquaculture pond or not. Describe what you see and compare and contrast it with the previous two known examples. Explain your thought process for classifying this image.

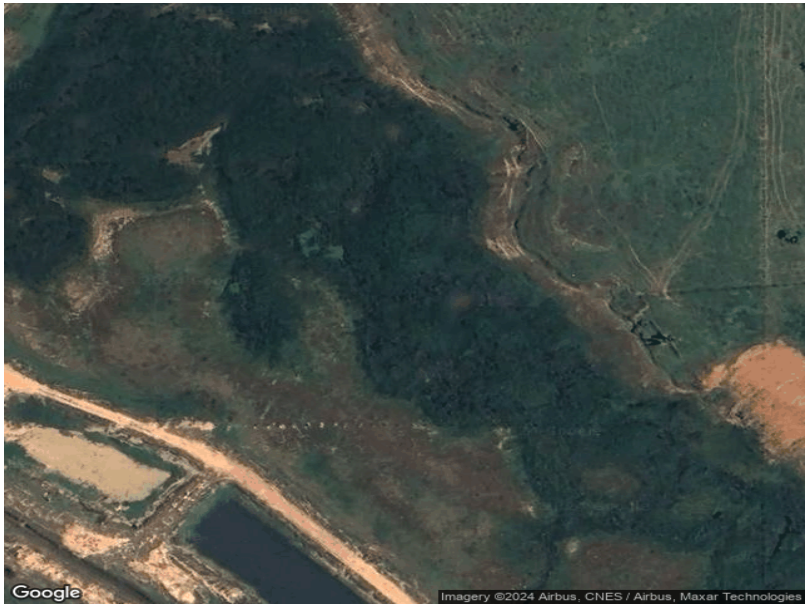

### Assistant:

In the provided satellite image, we need to determine whether there are aquaculture ponds present. Here is a detailed analysis and comparison with the previous examples:

#### Observations:

1. **Geometric Patterns:** In the lower left corner of the image, there are rectangular water bodies that exhibit straight edges and right angles, which are indicative of human-made structures.
2. **Water Color:** The water in these rectangular areas has a distinct color, different from the surrounding natural landscape, suggesting controlled water bodies.
3. **Surrounding Features:** There are visible access paths and possibly some infrastructure around the rectangular water bodies, which could be related to aquaculture operations.
4. **Location:** The rectangular water bodies are situated in an area that appears to be managed and possibly used for aquaculture, given the presence of infrastructure and access paths.
5. **Size and Scale:** The water bodies are uniform in size and shape, consistent with the organized nature of aquaculture ponds.
6. **Texture:** The water surfaces in the rectangular areas appear smooth, which is typical of controlled aquaculture ponds.

#### Comparison with Previous Examples:

- **Example with Aquaculture Pond:** The first example showed a clear rectangular pond with distinct water color and surrounding infrastructure. The current image has similar rectangular water bodies with distinct colors and surrounding features, suggesting aquaculture ponds.
- **Example without Aquaculture Pond:** The second example showed a natural landscape with dense vegetation and irregular water bodies. The current image, in contrast, has geometric water bodies and infrastructure, which are not present in the second example.

#### Thought Process for Classification:

1. **Geometric Shape:** The presence of rectangular water bodies with straight edges strongly suggests human-made ponds.
2. **Water Color and Texture:** The distinct color and smooth texture of the water bodies are consistent with aquaculture ponds.
3. **Surrounding Infrastructure:** The visible access paths and possible infrastructure support the idea of managed aquaculture operations.
4. **Comparison with Known Examples:** The current image shares more characteristics with the first example (with aquaculture pond) than the second example (without aquaculture pond).

## Conclusion:

Based on the geometric patterns, water color, surrounding features, and comparison with known examples, it is reasonable to classify this image as having aquaculture ponds. The rectangular water bodies with distinct characteristics and surrounding infrastructure are indicative of aquaculture operations.

## User:

You have access to the following tools to assist in your analysis: - PredictAquaculturePondTool: Tool Name: 'PredictAquaculturePondTool' Description: Predicts the probability of an aquaculture pond being present in the image using a machine learning model. This tool is particularly helpful when you need a quantitative assessment of the likelihood of aquaculture pond presence in the satellite image. The model has been trained on various satellite images of aquaculture ponds and provides a percentage probability. However, please note that the model can be wrong or inaccurate, especially in complex or ambiguous cases. It's important to use this tool's output as one piece of evidence among others, and not rely on it exclusively for your final decision. - PanUpToolRelative: Pans the view upwards relative to the last image seen. - PanUpToolAbsolute: Pans the view upwards relative to the original starting image. - PanDownToolRelative: Pans the view downwards relative to the last image seen. - PanDownToolAbsolute: Pans the view downwards relative to the original starting image. - PanLeftToolRelative: Pans the view to the left relative to the last image seen. - PanLeftToolAbsolute: Pans the view to the left relative to the original starting image. - PanRightToolRelative: Pans the view to the right relative to the last image seen. - PanRightToolAbsolute: Pans the view to the right relative to the original starting image. - ZoomInToolRelative: Zooms in on the center of the current view relative to the last image seen. - ZoomInToolAbsolute: Zooms in on the center of the original view relative to the original starting image. - ZoomOutToolRelative: Zooms out from the current view relative to the last image seen. - ZoomOutToolAbsolute: Zooms out from the original view relative to the original starting image.

You have 4 opportunities to use these tools. You are encouraged to use at least 3 tools to gather sufficient information. While it's good to conclude early if you're certain about the classification, the most important thing is making the correct prediction. Feel free to use more tools if you need to increase your confidence.

If you want to use a tool, explain how it will assist your analysis, then respond with the tool name in square brackets, like this: [ToolName], or if you are finished, respond with [Finished].

Remember, your goal is to accurately classify whether the image shows aquaculture ponds or not. If you do use a tool, you will see the result of the tool immediately, and you should briefly, 1-2 sentences describe any new insights from the tool, and your thoughts on the classification.

After each tool use, end your thought with brackets in the format {Yes:yesPercent,No:noPercent} to indicate your current confidence/prediction. For example, {Yes:70,No:30} would indicate 70% confidence in the presence of aquaculture ponds and 30% confidence in their absence. Note that this is not your final prediction.

Then you will be asked again if you want to use a tool or are finished.

## Assistant:

To start, I will use the PredictAquaculturePondTool to get a quantitative assessment of the likelihood of aquaculture ponds being present in the image. This will provide a baseline probability to inform my analysis.

[PredictAquaculturePondTool]

## User:

The probability of an aquaculture pond being present in this image is 25.91%. (Percentage out of 100%) Please note that this model has been trained on a limited dataset and its predictions can be inaccurate. Use this information as a guideline rather than a definitive prediction.

You have 3 rounds left. You may now choose another tool or indicate you're finished. Respond with ONLY [ToolName] to use a single tool, or [Finished] if you're done. Do not include multiple tool names or any other text in brackets. If you want to reference the last tool you used, simply write its name without brackets. After choosing a tool or indicating you're finished, provide your confidence in the presence of aquaculture ponds in the format {yes:PercentYes,no:PercentNo}. Then, explain why you are picking this tool or finishing, and how it relates to your current assessment of the image.

**Assistant:**

[ZoomInToolRelative]

{yes:60,no:40}

I am choosing to zoom in on the current view to get a closer look at the rectangular water bodies in the lower left corner. This will help me better assess their characteristics and determine if they are indeed aquaculture ponds.

**User:**

The view has been zoomed in, providing a closer look at the current view. New zoom level: 20

You have 2 rounds left. You may now choose another tool or indicate you're finished. Respond with ONLY [ToolName] to use a single tool, or [Finished] if you're done. Do not include multiple tool names or any other text in brackets. If you want to reference the last tool you used, simply write its name without brackets. After choosing a tool or indicating you're finished, provide your confidence in the presence of aquaculture ponds in the format {yes:PercentYes,no:PercentNo}. Then, explain why you are picking this tool or finishing, and how it relates to your current assessment of the image.

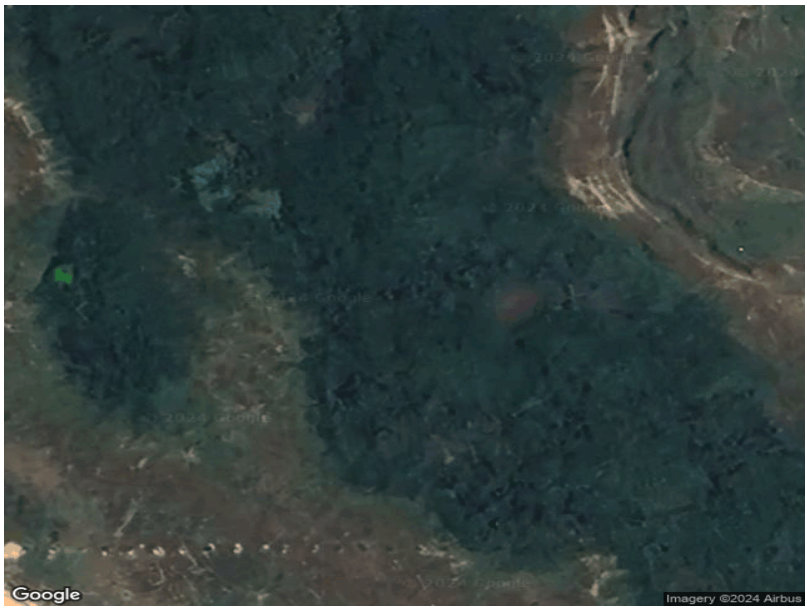

**Assistant:**

[PanDownToolRelative]

{yes:60,no:40}

I am choosing to pan down relative to the current view to get a better look at the rectangular water bodies that were partially visible in the lower left corner of the original image. This will help me confirm if they exhibit more characteristics of aquaculture ponds.

**User:**

The view has been panned down, revealing more of the area down of the previous view. New coordinates: Lat -10.337789827191068, Lon -62.823227003321655

You have 1 rounds left. You may now choose another tool or indicate you're finished. Respond with ONLY [ToolName] to use a single tool, or [Finished] if you're done. Do not include multiple tool names or any other text in brackets. If you want to reference the last tool you used, simply write its name without brackets. After choosing a tool or indicating you're finished, provide your confidence in the presence of aquaculture ponds in the format {yes:PercentYes,no:PercentNo}. Then, explain why you are picking this tool or finishing, and how it relates to your current assessment of the image.

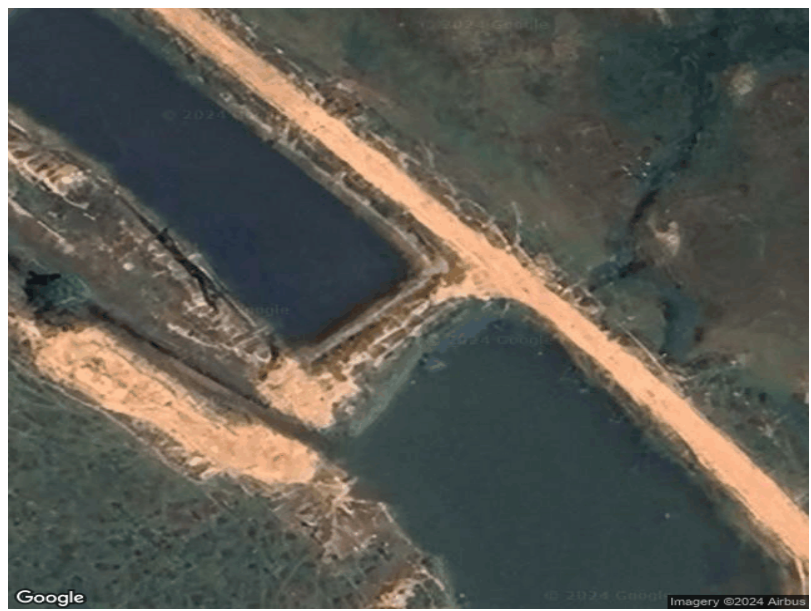

**Assistant:**

[ZoomInToolRelative]

{yes:80,no:20}

I am choosing to zoom in further on the current view to get a closer look at the rectangular water bodies. This will help me confirm the presence of aquaculture ponds by examining the details of the water bodies and surrounding infrastructure more closely.

**User:**

The view has been zoomed in, providing a closer look at the current view. New zoom level: 21

You have 0 rounds left. You may now choose another tool or indicate you're finished. Respond with ONLY [ToolName] to use a single tool, or [Finished] if you're done. Do not include multiple tool names or any other text in brackets. If you want to reference the last tool you used, simply write its name without brackets. After choosing a tool or indicating you're finished, provide your confidence in the presence of aquaculture ponds in the format {yes:PercentYes,no:PercentNo}. Then, explain why you are picking this tool or finishing, and how it relates to your current assessment of the image.

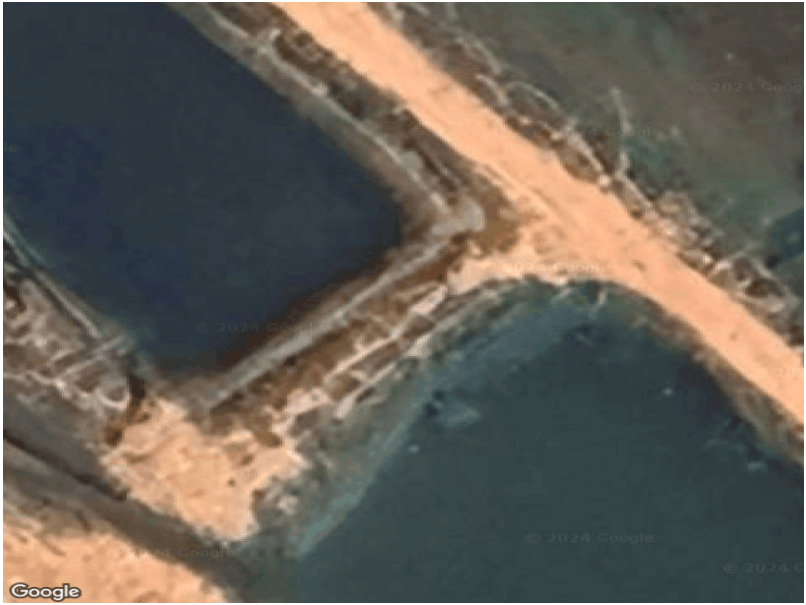

User:

Based on your analysis and the tools used, please provide your final classification regarding the presence of an aquaculture pond in the satellite image. Provide a brief explanation for your decision, including key observations and any tool results that influenced your conclusion. Consider the shape, color, and arrangement of water bodies, as well as any surrounding infrastructure that might indicate aquaculture activity. At the end of your response, you must provide your classification in the following format: [Yes:PercentYes,No:PercentNo], where PercentYes is the probability you think it is an aquaculture pond, and PercentNo is the probability you think it is not an aquaculture pond. These percentages must sum to 100%. To break ties, always assign at least 51% to one category. For example, [Yes:75,No:25] indicates 75% certainty of an aquaculture pond's presence, while [Yes:49,No:51] indicates 51% certainty of its absence.

Assistant:

Based on the analysis and the tools used, I conclude that the satellite image does show the presence of aquaculture ponds. Here are the key observations and tool results that influenced my decision:

1. **Geometric Patterns:** The water bodies in the image are rectangular with straight edges and right angles, which are indicative of human-made structures typical of aquaculture ponds.
2. **Water Color:** The water in these rectangular areas has a distinct color, different from the surrounding natural landscape, suggesting controlled water bodies.
3. **Surrounding Infrastructure:** There are visible access paths and infrastructure around the rectangular water bodies, which are consistent with aquaculture operations.
4. **PredictAquaculturePondTool:** Although the tool predicted a 25.91% probability of an aquaculture pond being present, this model's prediction is not definitive and should be used as a guideline. The visual evidence from the zoomed-in and panned views provides stronger support for the presence of aquaculture ponds.
5. **Zoom and Pan Tools:** The closer inspection provided by zooming in and panning down revealed more details of the rectangular water bodies and surrounding infrastructure, confirming their characteristics as aquaculture ponds.

Given these observations and the additional details obtained through the tools, I am confident in classifying the image as having aquaculture ponds.

Final classification: [Yes:80,No:20]
