# Supplementary material for: AiSciVision: A Framework for Specializing Large Multimodal Models in Scientific Image Classification
Source: arXiv:2410.21480 source file (2024-10-28)
Supplement: Supplementary file 2 [file solar_example.pdf]

True Class: 1, LMM Prediction: 1 (Probability: 0.99), Supervised Prediction: 1 (Probability: 98.95)

### System:

You are an expert in satellite imagery analysis specializing in solar panel detection. Your task is to determine whether a satellite image contains solar panels or not. Solar panels in satellite imagery typically appear as regular, geometric shapes with a distinct reflective surface. They are often arranged in arrays or grids on rooftops or in open fields. Key characteristics to look for include:

1. **Geometric Patterns:** Solar panels are usually arranged in rectangular or square shapes, forming distinct geometric patterns.
2. **Reflectivity:** Solar panels often appear brighter or more reflective than surrounding surfaces due to their glass or metal construction.
3. **Color Contrast:** Depending on the imagery, solar panels may appear darker or lighter than their surroundings, creating a noticeable contrast.
4. **Location:** Solar panels are commonly found on building rooftops, in open fields, or in designated solar farms.
5. **Size and Scale:** The size of solar panel arrays can vary greatly, from small rooftop installations to large utility-scale solar farms.

Use your knowledge and the tools provided to make an accurate classification of whether solar panels are present in the given satellite image.

### User:

This is an example of a satellite image containing solar panels. Describe what you see, focusing on the characteristics that indicate the presence of solar panels.

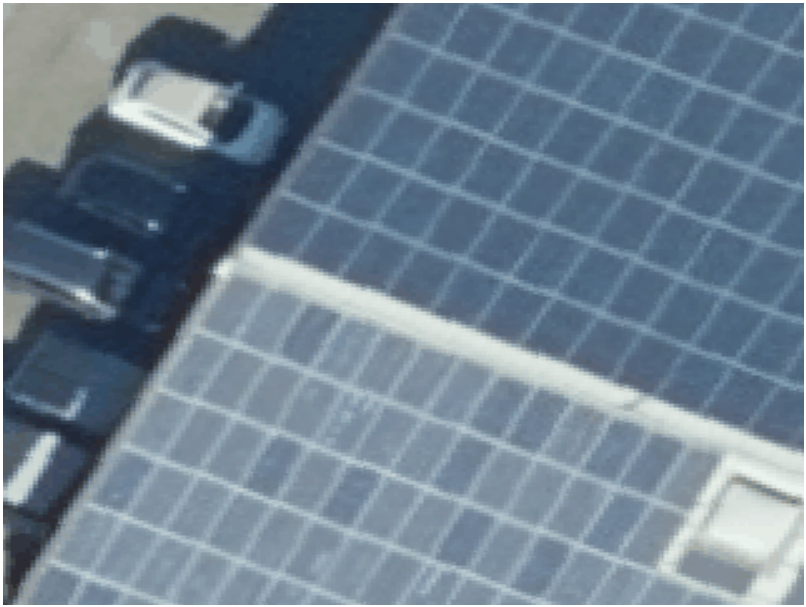

### Assistant:

In the provided satellite image, several characteristics indicate the presence of solar panels:

**Geometric Patterns:** The image shows a clear, regular grid pattern. The solar panels are arranged in a rectangular shape, which is typical for solar panel installations.

**Reflectivity:** The surface of the panels appears to have a distinct reflective quality, which is characteristic of the glass or metal materials used in solar panels.

**Color Contrast:** The panels have a uniform, darker color compared to the surrounding areas, creating a noticeable contrast. This contrast helps in distinguishing the solar panels from other objects or surfaces in the image.

**Location:** The panels are situated on what appears to be a rooftop, which is a common location for solar panel installations.

**Size and Scale:** The panels cover a significant portion of the rooftop, indicating a substantial installation, which is consistent with solar panel arrays.

These features collectively confirm that the image contains solar panels.

User:

This is an example of a satellite image without solar panels. Describe what you see, noting the absence of solar panels and any other relevant features.

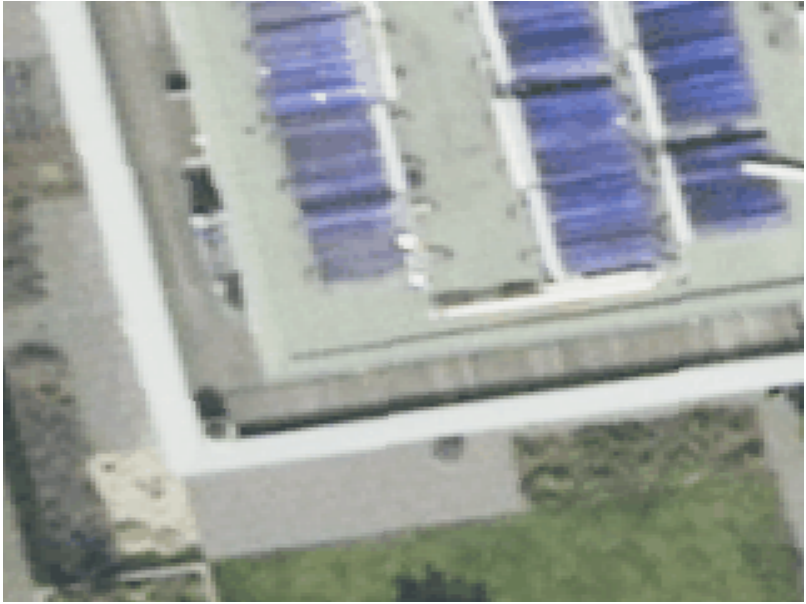

Assistant:

In the provided satellite image, several observations indicate the absence of solar panels:

**Geometric Patterns:** There are no distinct, regular grid patterns that are typical of solar panel installations. The structures on the rooftop do not exhibit the uniform rectangular or square shapes associated with solar panels.

**Reflectivity:** The surfaces in the image do not show the characteristic reflective quality of solar panels. Instead, the rooftop appears to have a more matte finish.

**Color Contrast:** While there are some darker and lighter areas on the rooftop, they do not form the consistent, uniform color contrast typical of solar panels. The darker areas seem to be more irregular and not indicative of solar panel arrays.

**Location:** The rooftop contains various structures, but none of them resemble the typical layout or appearance of solar panels. The structures could be HVAC units, skylights, or other rooftop equipment.

**Size and Scale:** The objects on the rooftop do not cover a significant portion in a manner consistent with solar panel installations. They appear to be scattered and varied in size.

Overall, the absence of the key characteristics of solar panels, such as geometric patterns, reflectivity, and uniform color contrast, confirms that this image does not contain solar panels. The rooftop instead features other types of equipment or structures.

User:

Here is the satellite image we need to classify as having solar panels or not. Describe what you see and compare and contrast it with the previous two known examples. Explain your thought process for classifying this image.

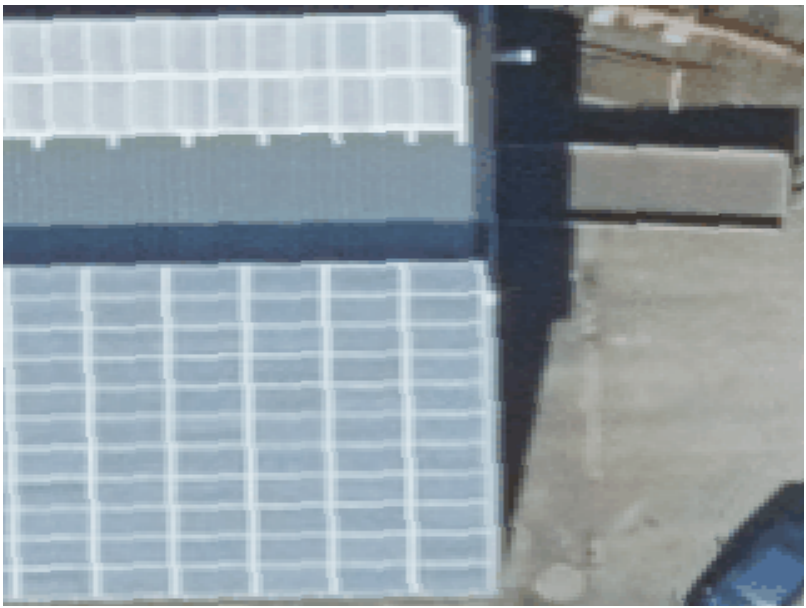

### Assistant:

In the provided satellite image, several characteristics suggest the presence of solar panels. Let's compare and contrast this image with the previous two examples to classify it accurately:

#### 1. **Geometric Patterns:**

- 2. **Current Image:** The image shows a clear, regular grid pattern with rectangular shapes, which is typical of solar panel installations.
- 3. **First Example (with solar panels):** Similar grid pattern and rectangular shapes are present.

**Second Example (without solar panels):** Lacks the regular grid pattern and rectangular shapes.

#### **Reflectivity:**

- 6. **Current Image:** The surfaces appear to have a reflective quality, consistent with the materials used in solar panels.
- 7. **First Example:** Reflective surfaces are evident.

**Second Example:** Reflective quality is absent, with a more matte finish.

#### **Color Contrast:**

- 10. **Current Image:** The panels have a uniform, lighter color compared to the surrounding areas, creating a noticeable contrast.
- 11. **First Example:** Similar uniform color contrast is present.

**Second Example:** Irregular color patterns without the uniform contrast typical of solar panels.

#### **Location:**

- 14. **Current Image:** The panels are situated on a rooftop, a common location for solar panel installations.
- 15. **First Example:** Panels are also on a rooftop.

**Second Example:** Various rooftop structures, but none resembling solar panels.

#### **Size and Scale:**

- 18. **Current Image:** The panels cover a significant portion of the rooftop, indicating a substantial installation.
- 19. **First Example:** Panels also cover a significant portion of the rooftop.
- 20. **Second Example:** Objects on the rooftop are scattered and varied in size, not consistent with solar panel arrays.

**Thought Process for Classification:** - The current image exhibits all the key characteristics of solar panels: geometric patterns, reflectivity, uniform color contrast, appropriate location, and significant coverage. - These characteristics align closely with the first example, which contains solar panels, and differ significantly from the second example, which does not contain solar panels.

Based on these observations, I classify the current image as containing solar panels.

### User:

You have access to the following tools to assist in your analysis: - PredictSolarPanelTool: Tool Name: 'PredictSolarPanelTool' Description: Predicts the probability of a solar panel being in the image using a machine learning model. This tool is particularly helpful when you need a quantitative assessment of the likelihood of a solar panel being present in the image. - HistogramEqualizationTool: Tool Name: 'HistogramEqualizationTool' Description: Enhances the contrast of the image using histogram equalization. This can help in making features more distinguishable, which is beneficial for detecting solar panels and potential defects. - AdjustBrightnessTool: Tool Name: 'AdjustBrightnessTool' Description: Adjusts the brightness of the image by 50%. This tool can help when the image is too dark or too bright, allowing for better visibility of solar panels and their features. - SharpenTool: Tool Name: 'SharpenTool' Description: Sharpens the image to enhance edges and details. This tool is useful for making subtle features more prominent, which can help in identifying solar panels and potential defects. - EdgeDetectionTool: Tool Name: 'EdgeDetectionTool' Description: Applies edge detection to the image, highlighting boundaries and features. This can help in identifying the outlines of solar panels and potential defects or anomalies. - IncreaseContrastTool: Tool Name: 'IncreaseContrastTool' Description: Increases the contrast of the image by 50%. This tool can be helpful when the image appears too flat or when you need to enhance the visibility of subtle details, especially in cases where solar panels might be hard to distinguish from their surroundings. - DecreaseContrastTool: Tool Name: 'DecreaseContrastTool' Description: Decreases the contrast of the image by 50%. This tool can be useful when the image appears too harsh or when you want to reduce the intensity of bright areas, which might help in identifying overall patterns or structures in the solar panel array.

You have 4 opportunities to use these tools. You are encouraged to use at least 3 tools to gather sufficient information. While it's good to conclude early if you're certain about the classification, the most important thing is making the correct prediction. Feel free to use more tools if you need to increase your confidence.

If you want to use a tool, explain how it will assist your analysis, then respond with the tool name in square brackets, like this: [ToolName], or if you are finished, respond with [Finished].

Remember, your goal is to accurately classify whether the image shows solar panels or not. If you do use a tool, you will see the result of the tool immediately, and you should briefly, 1-2 sentences describe any new insights from the tool, and your thoughts on the classification.

After each tool use, end your thought with brackets in the format {Yes:yesPercent,No:noPercent} to indicate your current confidence/prediction. For example, {Yes:70,No:30} would indicate 70% confidence in the presence of solar panels and 30% confidence in their absence. Note that this is not your final prediction.

Then you will be asked again if you want to use a tool or are finished.

### Assistant:

To start the analysis, I will use the **PredictSolarPanelTool** to get a quantitative assessment of the likelihood of solar panels being present in the image. This will provide a solid foundation for further analysis.

[PredictSolarPanelTool]

### User:

The probability of a solar panel being in this image is 98.95%. (Percentage out of 100%) Please note that this model has been trained on a limited dataset and its predictions can be inaccurate. Use this information as a guideline rather than a definitive prediction.

You have 3 rounds left. You may now choose another tool or indicate you're finished. Respond with ONLY [ToolName] to use a single tool, or [Finished] if you're done. Do not include multiple tool names or any other text in brackets. If you want to reference the last tool you used, simply write its name without brackets. After choosing a tool or indicating you're finished, provide your confidence in the presence of solar panels in the format {yes:PercentYes,no:PercentNo}. Then, explain why you are picking this tool or finishing, and

how it relates to your current assessment of the image.

**Assistant:**

[SharpenTool] {yes:98.95,no:1.05}

**User:**

Image sharpness has been increased.

You have 2 rounds left. You may now choose another tool or indicate you're finished. Respond with ONLY [ToolName] to use a single tool, or [Finished] if you're done. Do not include multiple tool names or any other text in brackets. If you want to reference the last tool you used, simply write its name without brackets. After choosing a tool or indicating you're finished, provide your confidence in the presence of solar panels in the format {yes:PercentYes,no:PercentNo}. Then, explain why you are picking this tool or finishing, and how it relates to your current assessment of the image.

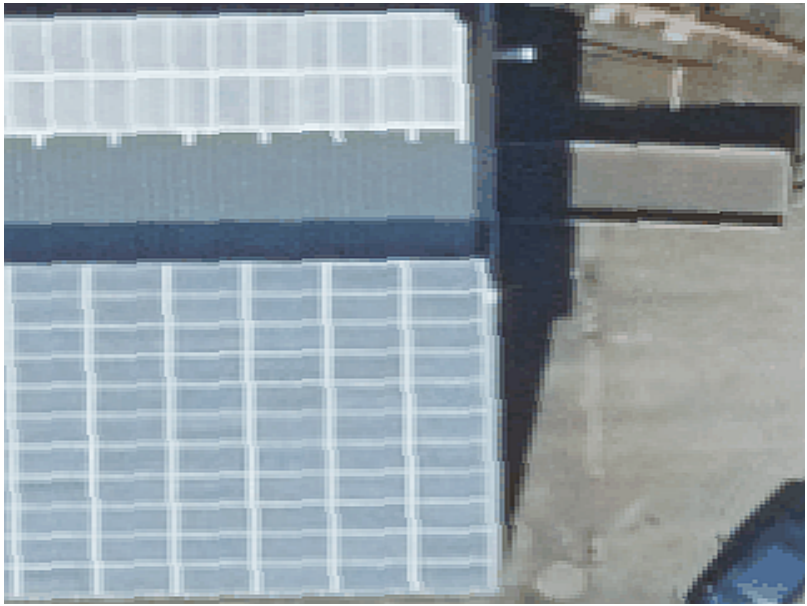

**Assistant:**

[EdgeDetectionTool] {yes:98.95,no:1.05}

**User:**

Edge detection has been applied to the image.

You have 1 rounds left. You may now choose another tool or indicate you're finished. Respond with ONLY [ToolName] to use a single tool, or [Finished] if you're done. Do not include multiple tool names or any other text in brackets. If you want to reference the last tool you used, simply write its name without brackets. After choosing a tool or indicating you're finished, provide your confidence in the presence of solar panels in the format {yes:PercentYes,no:PercentNo}. Then, explain why you are picking this tool or finishing, and how it relates to your current assessment of the image.

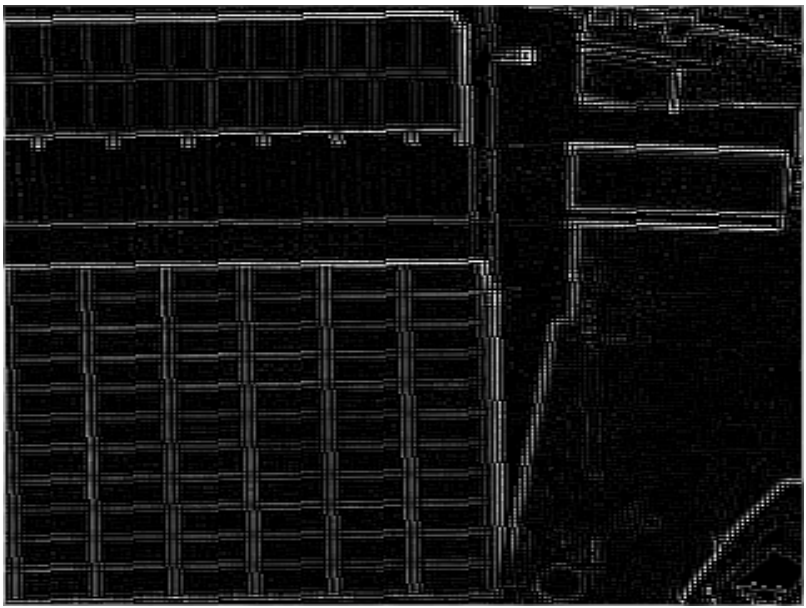

Assistant:

[HistogramEqualizationTool] {yes:98.95,no:1.05}

User:

Histogram equalization has been applied to enhance image contrast.

You have 0 rounds left. You may now choose another tool or indicate you're finished. Respond with ONLY [ToolName] to use a single tool, or [Finished] if you're done. Do not include multiple tool names or any other text in brackets. If you want to reference the last tool you used, simply write its name without brackets. After choosing a tool or indicating you're finished, provide your confidence in the presence of solar panels in the format {yes:PercentYes,no:PercentNo}. Then, explain why you are picking this tool or finishing, and how it relates to your current assessment of the image.

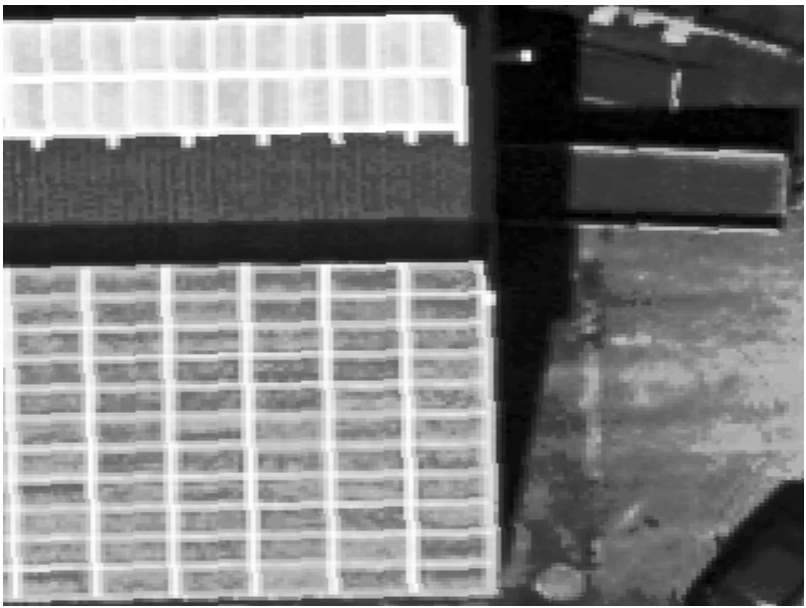

User:

Based on your analysis and the tools used, please provide your final classification regarding the presence of solar panels in the satellite image. Provide a brief explanation for your decision, including key observations and any tool results that influenced your conclusion. Consider the geometric patterns, reflectivity, color contrast, location, and size of potential solar panel installations. At the end of your response, you must provide your classification in the following format: [Yes:PercentYes,No:PercentNo], where PercentYes is the probability you think solar panels are present, and PercentNo is the probability you think they are not present. These

percentages must sum to 100%. To break ties, always assign at least 51% to one category. For example, [Yes:75,No:25] indicates 75% certainty of solar panel presence, while [Yes:49,No:51] indicates 51% certainty of their absence.

## Assistant:

Based on the analysis and the tools used, I conclude that the satellite image contains solar panels. Here are the key observations and tool results that influenced my decision:

**Geometric Patterns:** The image shows a clear, regular grid pattern with rectangular shapes, which is typical of solar panel installations. This was evident both before and after applying the SharpenTool and EdgeDetectionTool.

**Reflectivity:** The surfaces in the image appear to have a reflective quality, consistent with the materials used in solar panels. This was enhanced by the SharpenTool.

**Color Contrast:** The panels have a uniform, lighter color compared to the surrounding areas, creating a noticeable contrast. This was further highlighted by the HistogramEqualizationTool.

**Location:** The panels are situated on a rooftop, a common location for solar panel installations.

**Size and Scale:** The panels cover a significant portion of the rooftop, indicating a substantial installation.

The PredictSolarPanelTool provided a high probability (98.95%) of solar panels being present, which aligns with the visual analysis.

Final Classification: [Yes:99,No:1]

This high confidence is based on the consistent presence of key characteristics of solar panels across all tools and observations.
