# Supplementary material for: AiSciVision: A Framework for Specializing Large Multimodal Models in Scientific Image Classification
Source: arXiv:2410.21480 source file (2024-10-28)
Supplement: Supplementary file 3 [file visrag_tools_true1_lmm0_sup0.pdf]

True Class: 1, LMM Prediction: 0 (Probability: 0.40), Supervised Prediction: 0 (Probability: 7.13)

**System:**

You are an expert marine biologist specializing in eelgrass wasting disease classification. Your task is to determine whether an scan of an eelgrass blade contains eelgrass wasting disease or not. Eelgrass wasting disease, primarily caused by the marine pathogen *Labyrinthula zosterae*, presents visually as dark, necrotic lesions on the leaves of eelgrass (*Zostera marina*). These lesions typically appear as irregular black or brown spots or streaks, often starting at the tips of the leaves and spreading downwards. Over time, these lesions can coalesce, leading to extensive damage, including:

1. Spotting and Streaking: Initial symptoms include small, dark spots or streaks on the eelgrass leaves.
2. Blotching: As the disease progresses, these spots merge into larger blotches, which may appear dark brown or black.
3. Leaf Thinning and Loss: Affected areas may thin out or deteriorate, causing leaves to become more fragile and eventually break off.
4. Overall Decline: Heavily infected eelgrass beds often exhibit widespread dieback, with leaves appearing discolored, tattered, or decomposed.

Use your knowledge and the tools provided to make an accurate classification.

**User:**

I will start by first showing you an example image, that is visually similar to the image we want to classify, that does have eelgrass wasting disease. Then I will show you another example image that does not have eelgrass wasting disease, but is visually similar to the image we want to classify. Then I will show you the image we want to classify. For the first two, you should briefly (1-2 sentences) explain why it does or does not have eelgrass wasting disease. For the final image you should explain in a paragraph why you believe it does or does not have eelgrass wasting disease.

Here is the example that does have eelgrass wasting disease, only respond describing it, nothing else:

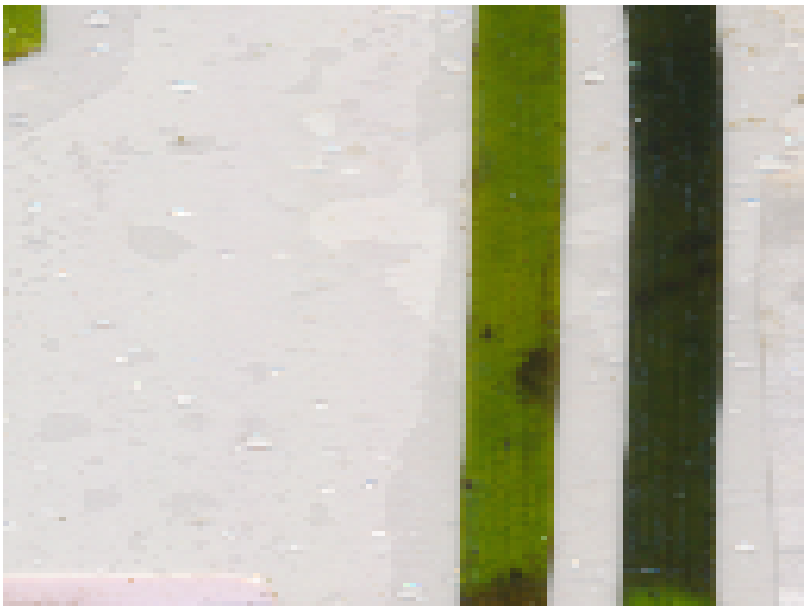

**Assistant:**

This image shows eelgrass blades with dark, necrotic lesions, which are indicative of eelgrass wasting disease. The irregular black or brown spots and streaks are visible, particularly starting from the tips and spreading downwards.

**User:**

Here is the example that does not have eelgrass wasting disease only respond describing it, nothing else:

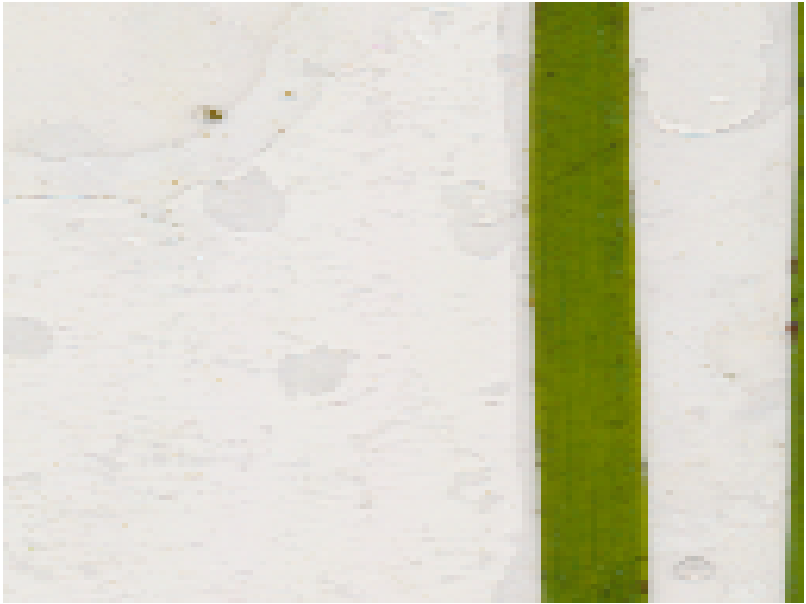

**Assistant:**

This image shows eelgrass blades that appear healthy, with no visible dark, necrotic lesions or irregular black or brown spots and streaks. The leaves are uniformly green and free from signs of eelgrass wasting disease.

**User:**

Here is the image need to classify as having eelgrass wasting disease or not. Describe what you see and compare and contrast it with the previous two known examples. Explain your thought process for classifying this image.

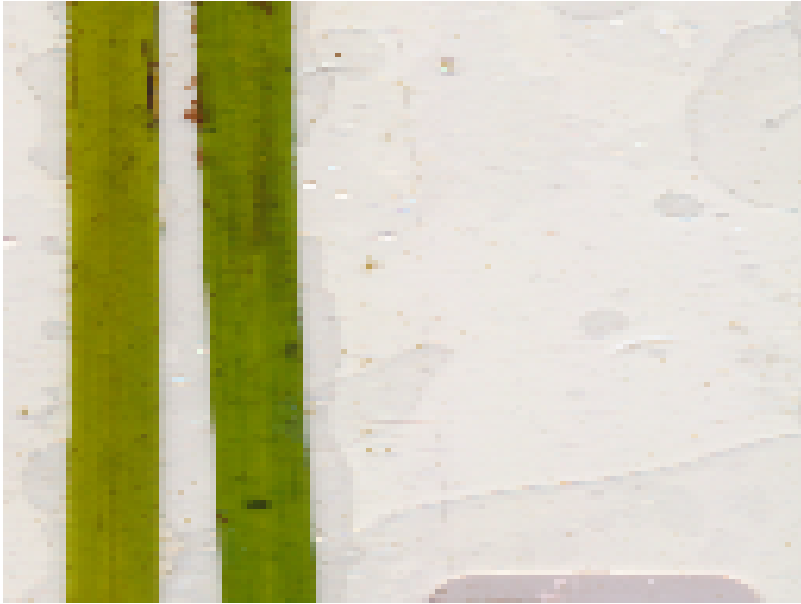

**Assistant:**

In this image, the eelgrass blades exhibit some dark spots and streaks, particularly towards the upper part of the blades. These dark areas are similar to the necrotic lesions seen in the first example image that had eelgrass wasting disease. The spots and streaks are irregular and appear to be spreading downwards, which is characteristic of the disease.

Comparing this image to the first example, the presence of dark, necrotic lesions is a common feature. In contrast, the second example image, which did not have eelgrass wasting disease, showed uniformly green and healthy blades without any dark spots or streaks.

Based on the presence of these dark, necrotic lesions and the pattern of spotting and streaking, I classify this image as having eelgrass wasting disease. The visual symptoms align closely with those seen in the diseased example, indicating that the eelgrass blades are affected by the disease.

**User:**

You have access to the following tools to assist in your analysis: - IncreaseContrastTool: Tool Name: 'IncreaseContrastTool' Description: Increases the contrast of the image by 50%. This tool can be helpful when the image appears too flat or when you need to enhance the visibility of subtle details, especially in cases where eelgrass wasting disease symptoms might be hard to distinguish. - DecreaseContrastTool: Tool Name: 'DecreaseContrastTool' Description: Decreases the contrast of the image by 50%. This tool can be useful when the image appears too harsh or when you want to reduce the intensity of bright areas, which might help in identifying overall patterns or structures in the eelgrass. - PredictEelgrassWastingDiseaseTool: Tool Name: 'PredictEelgrassWastingDiseaseTool' Description: Predicts the probability of eelgrass wasting disease in the image using a machine learning model. I recommend you use this tool. - AdjustBrightnessTool: Tool Name: 'AdjustBrightnessTool' Description: Adjusts the brightness of the image by 50%. This tool can help when the image is too dark or too bright, allowing for better visibility of disease symptoms on the eelgrass blade. - SharpenTool: Tool Name: 'SharpenTool' Description: Sharpens the image to enhance edges and details. This tool is useful for making subtle features more prominent, which can help in identifying signs of eelgrass wasting disease. - EdgeDetectionTool: Tool Name: 'EdgeDetectionTool' Description: Applies edge detection to the image, highlighting boundaries and features. This can help in identifying lesions or patterns associated with eelgrass wasting disease. - HistogramEqualizationTool: Tool Name: 'HistogramEqualizationTool' Description: Enhances the contrast of the image using histogram equalization. This can help in making features more distinguishable, which is beneficial for detecting eelgrass wasting disease symptoms.

You have 4 opportunities to use these tools. You are encouraged to use at least 3 tools to gather sufficient information. While it's good to conclude early if you're certain about the classification, the most important thing is making the correct prediction. Feel free to use more tools if you need to increase your confidence.

If you want to use a tool, explain how it will assist your analysis, then respond with the tool name in square brackets, like this: [ToolName], or if you are finished, respond with [Finished].

Remember, your goal is to accurately classify whether the image shows eelgrass wasting disease or not. If you do use a tool, you will see the result of the tool immediately, and you should briefly, 1-2 sentences describe any new insights from the tool, and your thoughts on the classification.

After each tool use, end your thought with brackets in the format {Yes:yesPercent,No:noPercent} to indicate your current confidence/prediction. For example, {Yes:70,No:30} would indicate 70% confidence in the presence of eelgrass wasting disease and 30% confidence in its absence. Note that this is not your final prediction.

Then you will be asked again if you want to use a tool or are finished.

**Assistant:**

To start, I will use the [IncreaseContrastTool] to enhance the visibility of any subtle details or lesions that might be present on the eelgrass blades. This will help in identifying any signs of eelgrass wasting disease more clearly.

[IncreaseContrastTool]

**User:**

Image contrast has been increased by 50%.

You have 3 rounds left. You may now choose another tool or indicate you're finished. Respond with ONLY [ToolName] to use a single tool, or [Finished] if you're done. Do not include multiple tool names or any other text in brackets. If you want to reference the last tool you used, simply write its name without brackets. After choosing a tool or indicating you're finished, provide your confidence in the presence of eelgrass wasting disease in the format {yes:PercentYes,no:PercentNo}. Then, explain why you are picking this tool or

finishing, and how it relates to your current assessment of the image.

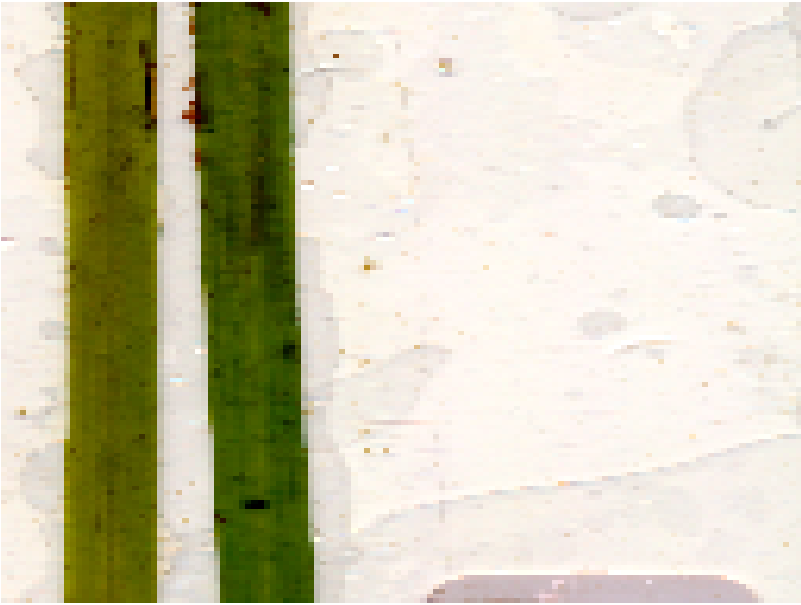

**Assistant:**

[SharpenTool]

{Yes:75,No:25}

I am using the SharpenTool to enhance the edges and details of the image further. This will help in making any subtle features, such as lesions or spots, more prominent, which can assist in identifying signs of eelgrass wasting disease more accurately.

**User:**

Image sharpness has been increased.

You have 2 rounds left. You may now choose another tool or indicate you're finished. Respond with ONLY [ToolName] to use a single tool, or [Finished] if you're done. Do not include multiple tool names or any other text in brackets. If you want to reference the last tool you used, simply write its name without brackets. After choosing a tool or indicating you're finished, provide your confidence in the presence of eelgrass wasting disease in the format {yes:PercentYes,no:PercentNo}. Then, explain why you are picking this tool or finishing, and how it relates to your current assessment of the image.

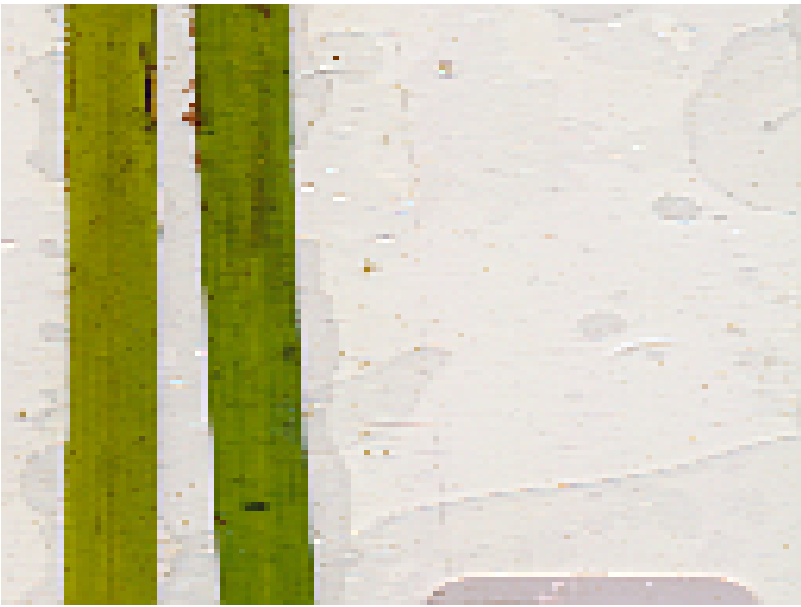

**Assistant:**

[PredictEelgrassWastingDiseaseTool]

{Yes:80,No:20}

I am using the PredictEelgrassWastingDiseaseTool to get a machine learning model's prediction on the probability of eelgrass wasting disease in the image. This will provide an additional layer of analysis and help confirm or refute my current assessment based on visual inspection.

**User:**

The probability of eelgrass wasting disease in this image is 7.13%. (Percentage out of 100%) Please note that this model has been trained on a limited dataset and its predictions can be inaccurate. Use this information as a guideline rather than a definitive diagnosis.

You have 1 rounds left. You may now choose another tool or indicate you're finished. Respond with ONLY [ToolName] to use a single tool, or [Finished] if you're done. Do not include multiple tool names or any other text in brackets. If you want to reference the last tool you used, simply write its name without brackets. After choosing a tool or indicating you're finished, provide your confidence in the presence of eelgrass wasting disease in the format {yes:PercentYes,no:PercentNo}. Then, explain why you are picking this tool or finishing, and how it relates to your current assessment of the image.

**Assistant:**

[EdgeDetectionTool]

{Yes:40,No:60}

I am using the EdgeDetectionTool to highlight boundaries and features in the image. This will help in identifying any lesions or patterns associated with eelgrass wasting disease more clearly, providing further evidence to support or refute the presence of the disease.

**User:**

Edge detection has been applied to the image.

You have 0 rounds left. You may now choose another tool or indicate you're finished. Respond with ONLY [ToolName] to use a single tool, or [Finished] if you're done. Do not include multiple tool names or any other text in brackets. If you want to reference the last tool you used, simply write its name without brackets. After choosing a tool or indicating you're finished, provide your confidence in the presence of eelgrass wasting disease in the format {yes:PercentYes,no:PercentNo}. Then, explain why you are picking this tool or finishing, and how it relates to your current assessment of the image.

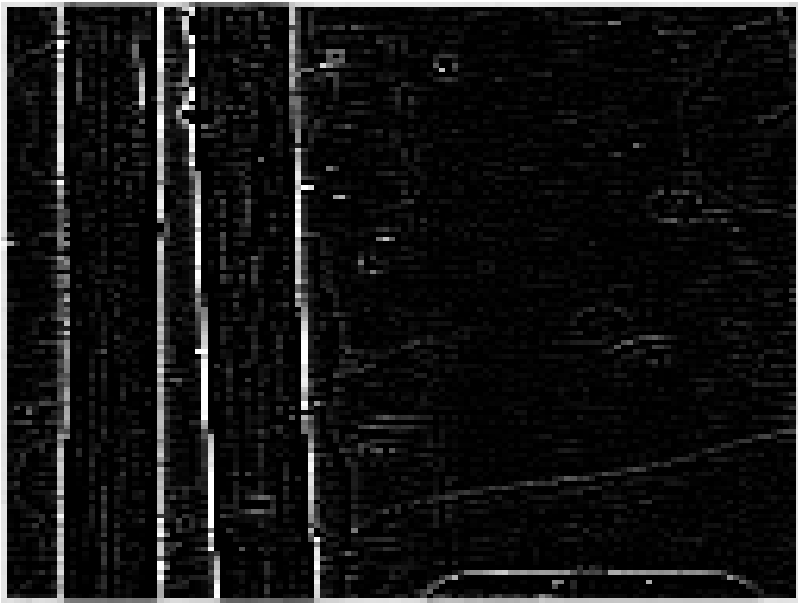

**User:**

Based on your analysis and the tools used, please provide your final classification regarding the presence of eelgrass wasting disease in the image. Provide a brief explanation for your decision, including key observations and any tool results that influenced your conclusion. Consider the color, texture, and pattern of the eelgrass leaves, as well as any visible lesions or discoloration that might indicate disease. At the end of your response, you must provide your classification in the following format: [Yes:PercentYes,No:PercentNo], where PercentYes is the probability you think eelgrass wasting disease is present, and PercentNo is the probability you think it is not present. These percentages must sum to 100%. To break ties, always assign at least 51% to one category. For example, [Yes:75,No:25] indicates 75% certainty of eelgrass wasting disease presence, while [Yes:49,No:51] indicates 51% certainty of its absence.

**Assistant:**

Based on the analysis and the tools used, I have made the following observations:

- Initial Visual Inspection:** The image showed some dark spots and streaks on the eelgrass blades, which initially suggested the presence of eelgrass wasting disease.
- IncreaseContrastTool:** This tool enhanced the visibility of subtle details, making the dark spots and streaks more prominent. This reinforced the initial suspicion of eelgrass wasting disease.
- SharpenTool:** This tool further enhanced the edges and details, making the dark spots and streaks even more noticeable. This continued to support the presence of the disease.
- PredictEelgrassWastingDiseaseTool:** The machine learning model predicted a low probability (7.13%) of eelgrass wasting disease. This result suggested that the visual signs might not be as indicative of the disease as initially thought.
- EdgeDetectionTool:** This tool highlighted the boundaries and features in the image. The detected edges did not show extensive or irregular patterns typically associated with severe eelgrass wasting disease lesions.

Considering all these observations, the initial visual signs of dark spots and streaks were not strongly supported by the machine learning model and the edge detection results. The low probability from the model and the lack of extensive irregular patterns in the edge detection suggest that the eelgrass blades might not be significantly affected by eelgrass wasting disease.

Final Classification: [Yes:40,No:60]

This indicates a 40% probability of eelgrass wasting disease presence and a 60% probability of its absence.
