# Supplementary material for: AiSciVision: A Framework for Specializing Large Multimodal Models in Scientific Image Classification
Source: arXiv:2410.21480 source file (2024-10-28)
Supplement: Supplementary file 4 [file eelgrass.pdf]

True Class: 1, LMM Prediction: 1 (Probability: 0.70), Supervised Prediction: 0 (Probability: 34.51)

### System:

You are an expert marine biologist specializing in eelgrass wasting disease classification. Your task is to determine whether an scan of an eelgrass blade contains eelgrass wasting disease or not. Eelgrass wasting disease, primarily caused by the marine pathogen *Labyrinthula zosterae*, presents visually as dark, necrotic lesions on the leaves of eelgrass (*Zostera marina*). These lesions typically appear as irregular black or brown spots or streaks, often starting at the tips of the leaves and spreading downwards. Over time, these lesions can coalesce, leading to extensive damage, including:

1. Spotting and Streaking: Initial symptoms include small, dark spots or streaks on the eelgrass leaves.
2. Blotching: As the disease progresses, these spots merge into larger blotches, which may appear dark brown or black.
3. Leaf Thinning and Loss: Affected areas may thin out or deteriorate, causing leaves to become more fragile and eventually break off.
4. Overall Decline: Heavily infected eelgrass beds often exhibit widespread dieback, with leaves appearing discolored, tattered, or decomposed.

Use your knowledge and the tools provided to make an accurate classification.

### User:

I will start by first showing you an example image, that is visually similar to the image we want to classify, that does have eelgrass wasting disease. Then I will show you another example image that does not have eelgrass wasting disease, but is visually similar to the image we want to classify. Then I will show you the image we want to classify. For the first two, you should briefly (1-2 sentences) explain why it does or does not have eelgrass wasting disease. For the final image you should explain in a paragraph why you believe it does or does not have eelgrass wasting disease.

Here is the example that does have eelgrass wasting disease, only respond describing it, nothing else:

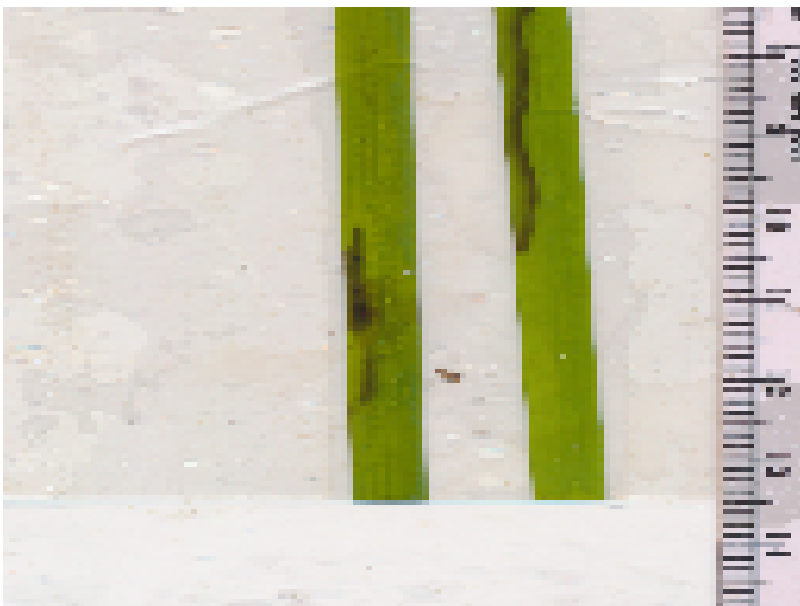

### Assistant:

This image shows eelgrass blades with dark, necrotic lesions. The lesions appear as irregular black or brown spots and streaks, indicative of eelgrass wasting disease.

### User:

Here is the example that does not have eelgrass wasting disease only respond describing it, nothing else:

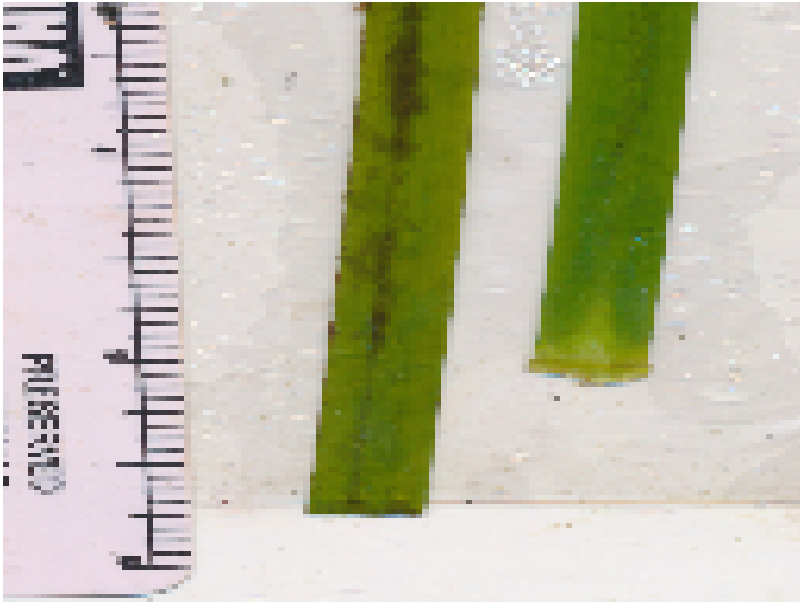

**Assistant:**

This image shows eelgrass blades that are uniformly green without any dark, necrotic lesions or irregular black or brown spots, indicating the absence of eelgrass wasting disease.

**User:**

Here is the image need to classify as having eelgrass wasting disease or not. Describe what you see and compare and contrast it with the previous two known examples. Explain your thought process for classifying this image.

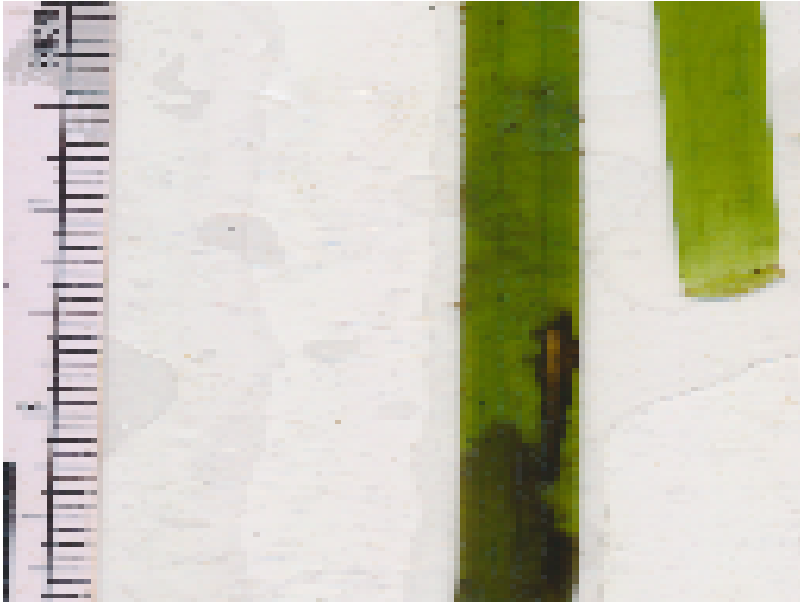

**Assistant:**

This image shows eelgrass blades, one of which has a dark, necrotic lesion near the base. The lesion appears as an irregular black or brown spot, similar to the lesions seen in the first example image that had eelgrass wasting disease. The other blade appears uniformly green without any visible lesions.

Comparing this image to the first example, the presence of dark, necrotic lesions on one of the blades is consistent with the symptoms of eelgrass wasting disease. In contrast, the second example image, which did not have the disease, showed uniformly green blades without any dark spots or streaks.

Based on the presence of the dark, necrotic lesion on one of the blades in this image, it is likely that this eelgrass blade is affected by eelgrass wasting disease. The lesion's appearance and location are characteristic of the disease, supporting this classification.

## User:

You have access to the following tools to assist in your analysis: - IncreaseContrastTool: Tool Name: 'IncreaseContrastTool' Description: Increases the contrast of the image by 50%. This tool can be helpful when the image appears too flat or when you need to enhance the visibility of subtle details, especially in cases where eelgrass wasting disease symptoms might be hard to distinguish. - DecreaseContrastTool: Tool Name: 'DecreaseContrastTool' Description: Decreases the contrast of the image by 50%. This tool can be useful when the image appears too harsh or when you want to reduce the intensity of bright areas, which might help in identifying overall patterns or structures in the eelgrass. - PredictEelgrassWastingDiseaseTool: Tool Name: 'PredictEelgrassWastingDiseaseTool' Description: Predicts the probability of eelgrass wasting disease in the image using a machine learning model. I recommend you use this tool. - AdjustBrightnessTool: Tool Name: 'AdjustBrightnessTool' Description: Adjusts the brightness of the image by 50%. This tool can help when the image is too dark or too bright, allowing for better visibility of disease symptoms on the eelgrass blade. - SharpenTool: Tool Name: 'SharpenTool' Description: Sharpens the image to enhance edges and details. This tool is useful for making subtle features more prominent, which can help in identifying signs of eelgrass wasting disease. - EdgeDetectionTool: Tool Name: 'EdgeDetectionTool' Description: Applies edge detection to the image, highlighting boundaries and features. This can help in identifying lesions or patterns associated with eelgrass wasting disease. - HistogramEqualizationTool: Tool Name: 'HistogramEqualizationTool' Description: Enhances the contrast of the image using histogram equalization. This can help in making features more distinguishable, which is beneficial for detecting eelgrass wasting disease symptoms.

You have 4 opportunities to use these tools. You are encouraged to use at least 3 tools to gather sufficient information. While it's good to conclude early if you're certain about the classification, the most important thing is making the correct prediction. Feel free to use more tools if you need to increase your confidence.

If you want to use a tool, explain how it will assist your analysis, then respond with the tool name in square brackets, like this: [ToolName], or if you are finished, respond with [Finished].

Remember, your goal is to accurately classify whether the image shows eelgrass wasting disease or not. If you do use a tool, you will see the result of the tool immediately, and you should briefly, 1-2 sentences describe any new insights from the tool, and your thoughts on the classification.

After each tool use, end your thought with brackets in the format {Yes:yesPercent,No:noPercent} to indicate your current confidence/prediction. For example, {Yes:70,No:30} would indicate 70% confidence in the presence of eelgrass wasting disease and 30% confidence in its absence. Note that this is not your final prediction.

Then you will be asked again if you want to use a tool or are finished.

## Assistant:

To start, I will use the [IncreaseContrastTool] to enhance the visibility of any subtle details in the image, which might help in identifying the presence of eelgrass wasting disease symptoms more clearly.

[IncreaseContrastTool]

## User:

Image contrast has been increased by 50%.

You have 3 rounds left. You may now choose another tool or indicate you're finished. Respond with ONLY [ToolName] to use a single tool, or [Finished] if you're done. Do not include multiple tool names or any other text in brackets. If you want to reference the last tool you used, simply write its name without brackets. After choosing a tool or indicating you're finished, provide your confidence in the presence of eelgrass wasting disease in the format {yes:PercentYes,no:PercentNo}. Then, explain why you are picking this tool or finishing, and how it relates to your current assessment of the image.

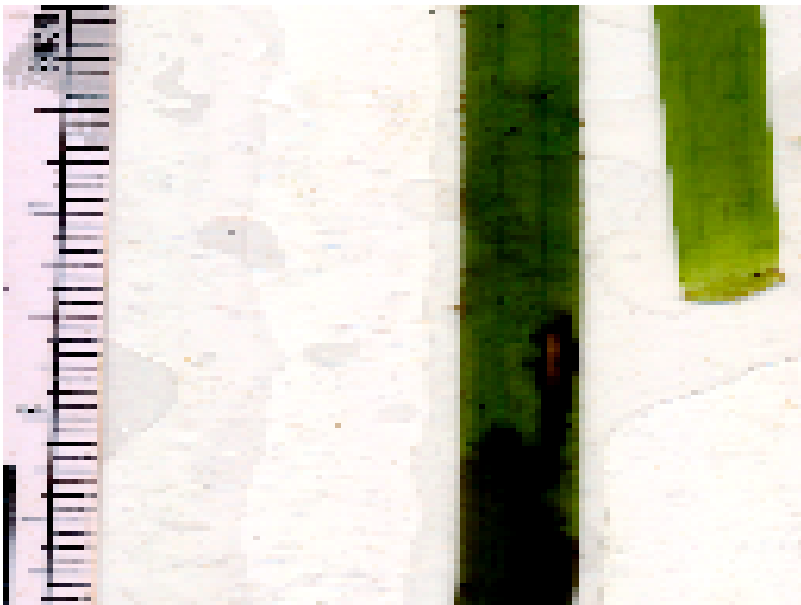

Assistant:

{yes:80,no:20}

The increased contrast has made the dark, necrotic lesion more prominent, reinforcing the initial observation that this blade might be affected by eelgrass wasting disease. To further enhance the visibility of the lesion and confirm its characteristics, I will use the [SharpenTool] to make the edges and details more prominent.

[SharpenTool]

User:

Image sharpness has been increased.

You have 2 rounds left. You may now choose another tool or indicate you're finished. Respond with ONLY [ToolName] to use a single tool, or [Finished] if you're done. Do not include multiple tool names or any other text in brackets. If you want to reference the last tool you used, simply write its name without brackets. After choosing a tool or indicating you're finished, provide your confidence in the presence of eelgrass wasting disease in the format {yes:PercentYes,no:PercentNo}. Then, explain why you are picking this tool or finishing, and how it relates to your current assessment of the image.

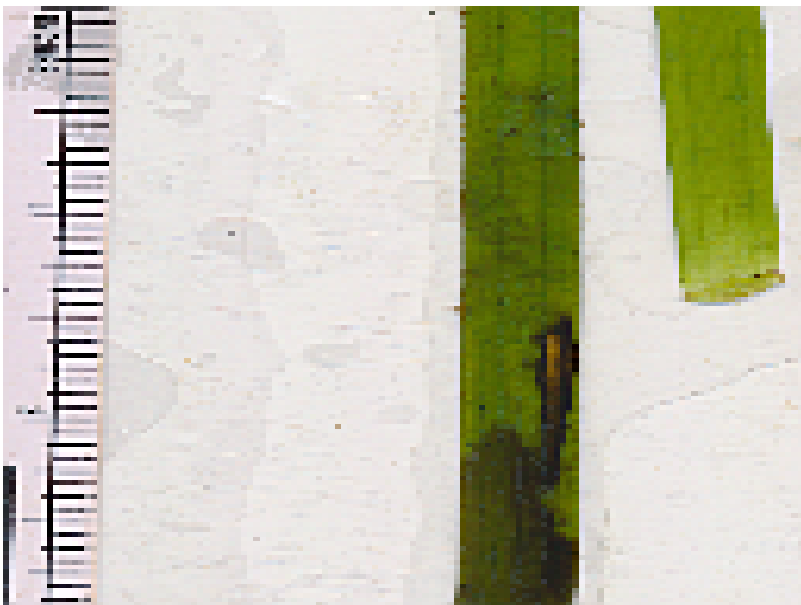

Assistant:

{yes:85,no:15}

The sharpening has further clarified the edges and details of the dark lesion, making it more evident that the lesion is consistent with the symptoms of eelgrass wasting disease. To solidify my assessment, I will use the [PredictEelgrassWastingDiseaseTool] to get a probability prediction from a machine learning model.

[PredictEelgrassWastingDiseaseTool]

**User:**

The probability of eelgrass wasting disease in this image is 34.51%. (Percentage out of 100%) Please note that this model has been trained on a limited dataset and its predictions can be inaccurate. Use this information as a guideline rather than a definitive diagnosis.

You have 1 rounds left. You may now choose another tool or indicate you're finished. Respond with ONLY [ToolName] to use a single tool, or [Finished] if you're done. Do not include multiple tool names or any other text in brackets. If you want to reference the last tool you used, simply write its name without brackets. After choosing a tool or indicating you're finished, provide your confidence in the presence of eelgrass wasting disease in the format {yes:PercentYes,no:PercentNo}. Then, explain why you are picking this tool or finishing, and how it relates to your current assessment of the image.

**Assistant:**

{yes:70,no:30}

The machine learning model's prediction of a 34.51% probability of eelgrass wasting disease suggests some uncertainty. To further enhance the visibility of any subtle details and make a more informed decision, I will use the [HistogramEqualizationTool] to improve the contrast and distinguishability of features in the image.

[HistogramEqualizationTool]

**User:**

Histogram equalization has been applied to enhance image contrast.

You have 0 rounds left. You may now choose another tool or indicate you're finished. Respond with ONLY [ToolName] to use a single tool, or [Finished] if you're done. Do not include multiple tool names or any other text in brackets. If you want to reference the last tool you used, simply write its name without brackets. After choosing a tool or indicating you're finished, provide your confidence in the presence of eelgrass wasting disease in the format {yes:PercentYes,no:PercentNo}. Then, explain why you are picking this tool or finishing, and how it relates to your current assessment of the image.

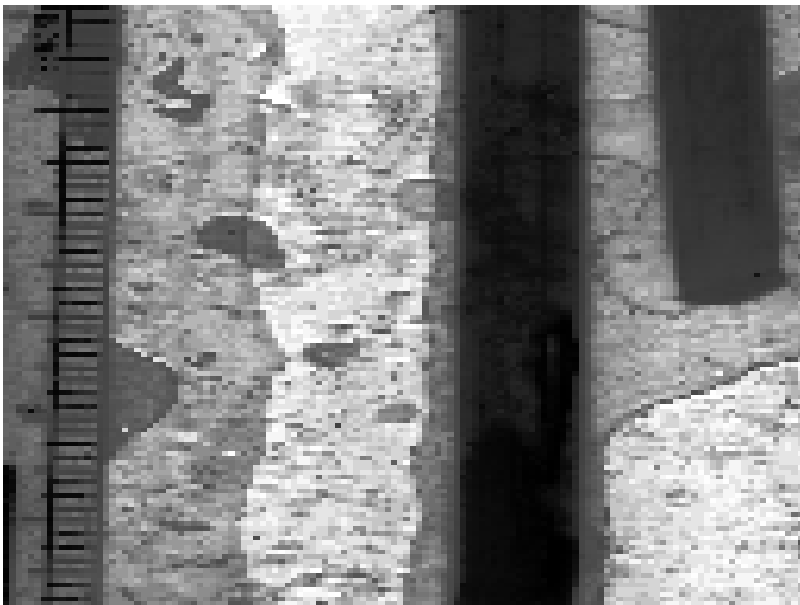

User:

Based on your analysis and the tools used, please provide your final classification regarding the presence of eelgrass wasting disease in the image. Provide a brief explanation for your decision, including key observations and any tool results that influenced your conclusion. Consider the color, texture, and pattern of the eelgrass leaves, as well as any visible lesions or discoloration that might indicate disease. At the end of your response, you must provide your classification in the following format:

[Yes:PercentYes,No:PercentNo], where PercentYes is the probability you think eelgrass wasting disease is present, and PercentNo is the probability you think it is not present. These percentages must sum to 100%. To break ties, always assign at least 51% to one category. For example, [Yes:75,No:25] indicates 75% certainty of eelgrass wasting disease presence, while [Yes:49,No:51] indicates 51% certainty of its absence.

Assistant:

Based on the analysis and the tools used, the final classification regarding the presence of eelgrass wasting disease in the image is as follows:

1. **Initial Observation:** The image initially showed a dark, necrotic lesion on one of the eelgrass blades, which is a characteristic symptom of eelgrass wasting disease.
2. **IncreaseContrastTool:** This tool enhanced the visibility of the lesion, making it more prominent and consistent with the symptoms of eelgrass wasting disease.
3. **SharpenTool:** The sharpening further clarified the edges and details of the lesion, reinforcing the initial observation.
4. **PredictEelgrassWastingDiseaseTool:** The machine learning model predicted a 34.51% probability of eelgrass wasting disease, suggesting some uncertainty but not ruling out the presence of the disease.
5. **HistogramEqualizationTool:** This tool improved the contrast and distinguishability of features in the image, making the lesion more visible and confirming its irregular shape and dark coloration.

Considering the consistent presence of a dark, necrotic lesion on one of the eelgrass blades, which aligns with the symptoms of eelgrass wasting disease, and despite the machine learning model's lower probability, the visual evidence strongly suggests the presence of the disease.

Final Classification: [Yes:70,No:30]

This indicates a 70% certainty of eelgrass wasting disease presence based on the visual analysis and tool results.
