# Supplementary material for: AiSciVision: A Framework for Specializing Large Multimodal Models in Scientific Image Classification
Source: arXiv:2410.21480 source file (2024-10-28)
Supplement: Supplementary file 5 [file tools_true1_lmm0_sup0.pdf]

True Class: 1, LMM Prediction: 0 (Probability: 0.20), Supervised Prediction: 0 (Probability: 7.13)

### System:

You are an expert marine biologist specializing in eelgrass wasting disease classification. Your task is to determine whether an scan of an eelgrass blade contains eelgrass wasting disease or not. Eelgrass wasting disease, primarily caused by the marine pathogen *Labyrinthula zosterae*, presents visually as dark, necrotic lesions on the leaves of eelgrass (*Zostera marina*). These lesions typically appear as irregular black or brown spots or streaks, often starting at the tips of the leaves and spreading downwards. Over time, these lesions can coalesce, leading to extensive damage, including:

1. Spotting and Streaking: Initial symptoms include small, dark spots or streaks on the eelgrass leaves.
2. Blotching: As the disease progresses, these spots merge into larger blotches, which may appear dark brown or black.
3. Leaf Thinning and Loss: Affected areas may thin out or deteriorate, causing leaves to become more fragile and eventually break off.
4. Overall Decline: Heavily infected eelgrass beds often exhibit widespread dieback, with leaves appearing discolored, tattered, or decomposed.

Use your knowledge and the tools provided to make an accurate classification.

### User:

Here is the image we want to classify. Explain your thought process for classifying this image.

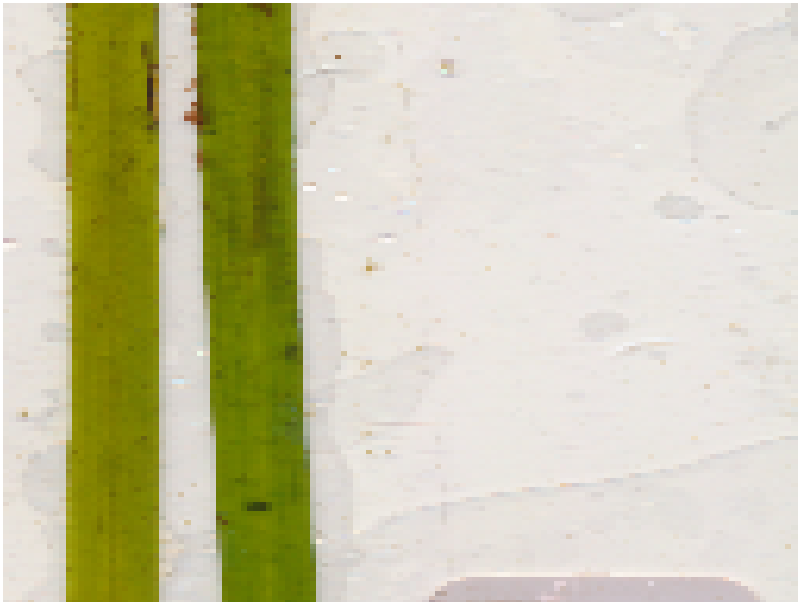

### Assistant:

To classify this image for eelgrass wasting disease, I will follow these steps:

**Identify Dark Spots or Streaks:** Look for any small, dark spots or streaks on the eelgrass leaves. These are initial symptoms of the disease.

**Check for Blotching:** Determine if these spots have merged into larger blotches, which may appear dark brown or black.

**Assess Leaf Thinning and Loss:** Examine if the affected areas are thinning out or deteriorating, causing the leaves to become more fragile.

**Overall Condition:** Evaluate the overall condition of the eelgrass leaves to see if there is widespread dieback, discoloration, or decomposition.

### Analysis of the Image:

**Dark Spots or Streaks:** The image shows two eelgrass blades. The blade on the left has a dark streak running down its length, which is a potential indicator of the initial symptoms of eelgrass wasting disease.

**Blotching:** The dark streak on the left blade does not appear to have merged into larger blotches, but it is a significant dark streak.

**Leaf Thinning and Loss:** There is no clear evidence of leaf thinning or loss in the image. The blades appear intact and not fragile.

**Overall Condition:** The overall condition of the eelgrass blades seems relatively healthy, except for the dark streak on the left blade.

## Conclusion:

Based on the presence of a dark streak on the left blade, it is possible that this eelgrass blade is in the early stages of eelgrass wasting disease. However, the absence of extensive blotching, leaf thinning, and overall dieback suggests that the disease may not be in an advanced stage.

Therefore, I would classify this image as showing early signs of eelgrass wasting disease.

## User:

You have access to the following tools to assist in your analysis: - IncreaseContrastTool: Tool Name: 'IncreaseContrastTool' Description: Increases the contrast of the image by 50%. This tool can be helpful when the image appears too flat or when you need to enhance the visibility of subtle details, especially in cases where eelgrass wasting disease symptoms might be hard to distinguish. - DecreaseContrastTool: Tool Name: 'DecreaseContrastTool' Description: Decreases the contrast of the image by 50%. This tool can be useful when the image appears too harsh or when you want to reduce the intensity of bright areas, which might help in identifying overall patterns or structures in the eelgrass. - PredictEelgrassWastingDiseaseTool: Tool Name: 'PredictEelgrassWastingDiseaseTool' Description: Predicts the probability of eelgrass wasting disease in the image using a machine learning model. I recommend you use this tool. - AdjustBrightnessTool: Tool Name: 'AdjustBrightnessTool' Description: Adjusts the brightness of the image by 50%. This tool can help when the image is too dark or too bright, allowing for better visibility of disease symptoms on the eelgrass blade. - SharpenTool: Tool Name: 'SharpenTool' Description: Sharpens the image to enhance edges and details. This tool is useful for making subtle features more prominent, which can help in identifying signs of eelgrass wasting disease. - EdgeDetectionTool: Tool Name: 'EdgeDetectionTool' Description: Applies edge detection to the image, highlighting boundaries and features. This can help in identifying lesions or patterns associated with eelgrass wasting disease. - HistogramEqualizationTool: Tool Name: 'HistogramEqualizationTool' Description: Enhances the contrast of the image using histogram equalization. This can help in making features more distinguishable, which is beneficial for detecting eelgrass wasting disease symptoms.

You have 4 opportunities to use these tools. You are encouraged to use at least 3 tools to gather sufficient information. While it's good to conclude early if you're certain about the classification, the most important thing is making the correct prediction. Feel free to use more tools if you need to increase your confidence.

If you want to use a tool, explain how it will assist your analysis, then respond with the tool name in square brackets, like this: [ToolName], or if you are finished, respond with [Finished].

Remember, your goal is to accurately classify whether the image shows eelgrass wasting disease or not. If you do use a tool, you will see the result of the tool immediately, and you should briefly, 1-2 sentences describe any new insights from the tool, and your thoughts on the classification.

After each tool use, end your thought with brackets in the format {Yes:yesPercent,No:noPercent} to indicate your current confidence/prediction. For example, {Yes:70,No:30} would indicate 70% confidence in the presence of eelgrass wasting disease and 30% confidence in its absence. Note that this is not your final prediction.

Then you will be asked again if you want to use a tool or are finished.

## Assistant:

To start, I will use the [IncreaseContrastTool] to enhance the visibility of any subtle details that might indicate the presence of eelgrass wasting disease. This will help in identifying any dark spots, streaks, or blotches more clearly.

[IncreaseContrastTool]

**User:**

Image contrast has been increased by 50%.

You have 3 rounds left. You may now choose another tool or indicate you're finished. Respond with ONLY [ToolName] to use a single tool, or [Finished] if you're done. Do not include multiple tool names or any other text in brackets. If you want to reference the last tool you used, simply write its name without brackets. After choosing a tool or indicating you're finished, provide your confidence in the presence of eelgrass wasting disease in the format {yes:PercentYes,no:PercentNo}. Then, explain why you are picking this tool or finishing, and how it relates to your current assessment of the image.

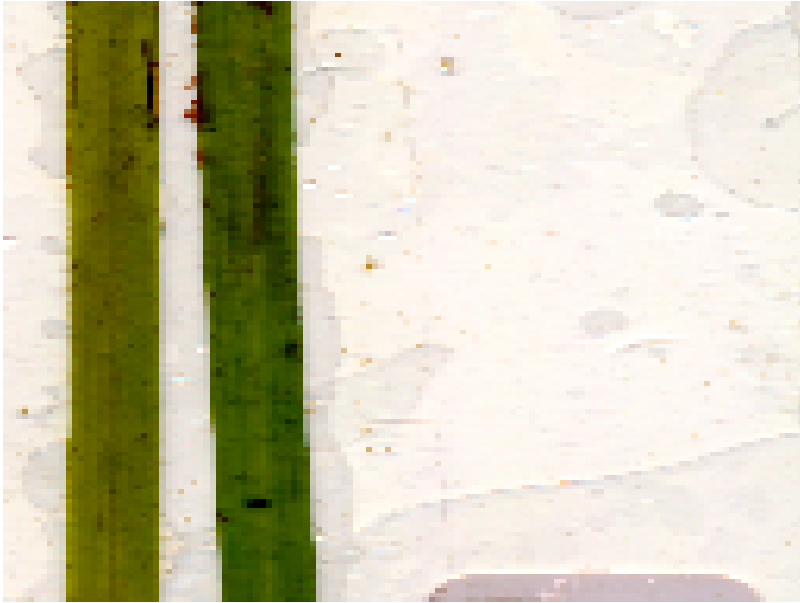

**Assistant:**

[SharpenTool]

{yes:60,no:40}

I am using the SharpenTool to enhance the edges and details of the image further. This will help in making any subtle features, such as dark spots or streaks, more prominent, which can assist in identifying signs of eelgrass wasting disease.

**User:**

Image sharpness has been increased.

You have 2 rounds left. You may now choose another tool or indicate you're finished. Respond with ONLY [ToolName] to use a single tool, or [Finished] if you're done. Do not include multiple tool names or any other text in brackets. If you want to reference the last tool you used, simply write its name without brackets. After choosing a tool or indicating you're finished, provide your confidence in the presence of eelgrass wasting disease in the format {yes:PercentYes,no:PercentNo}. Then, explain why you are picking this tool or finishing, and how it relates to your current assessment of the image.

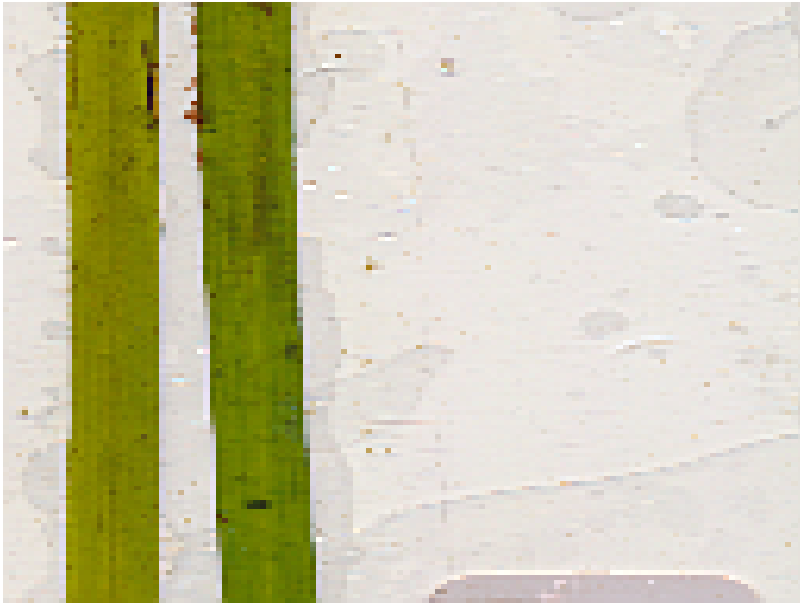

**Assistant:**

[PredictEelgrassWastingDiseaseTool]

{yes:65,no:35}

I am using the PredictEelgrassWastingDiseaseTool to leverage a machine learning model that can provide a probability of eelgrass wasting disease in the image. This will help in confirming or adjusting my current assessment based on the enhanced visibility from the previous tools.

**User:**

The probability of eelgrass wasting disease in this image is 7.13%. (Percentage out of 100%) Please note that this model has been trained on a limited dataset and its predictions can be inaccurate. Use this information as a guideline rather than a definitive diagnosis.

You have 1 rounds left. You may now choose another tool or indicate you're finished. Respond with ONLY [ToolName] to use a single tool, or [Finished] if you're done. Do not include multiple tool names or any other text in brackets. If you want to reference the last tool you used, simply write its name without brackets. After choosing a tool or indicating you're finished, provide your confidence in the presence of eelgrass wasting disease in the format {yes:PercentYes,no:PercentNo}. Then, explain why you are picking this tool or finishing, and how it relates to your current assessment of the image.

**Assistant:**

[EdgeDetectionTool]

{yes:20,no:80}

I am using the EdgeDetectionTool to highlight boundaries and features in the image. This will help in identifying any lesions or patterns associated with eelgrass wasting disease more clearly, which can further confirm or refute the low probability suggested by the PredictEelgrassWastingDiseaseTool.

**User:**

Edge detection has been applied to the image.

You have 0 rounds left. You may now choose another tool or indicate you're finished. Respond with ONLY [ToolName] to use a single tool, or [Finished] if you're done. Do not include multiple tool names or any other text in brackets. If you want to reference the last tool you used, simply write its name without brackets. After choosing a tool or indicating you're finished, provide your confidence in the presence of eelgrass wasting disease in the format {yes:PercentYes,no:PercentNo}. Then, explain why you are picking this tool or finishing, and how it relates to your current assessment of the image.

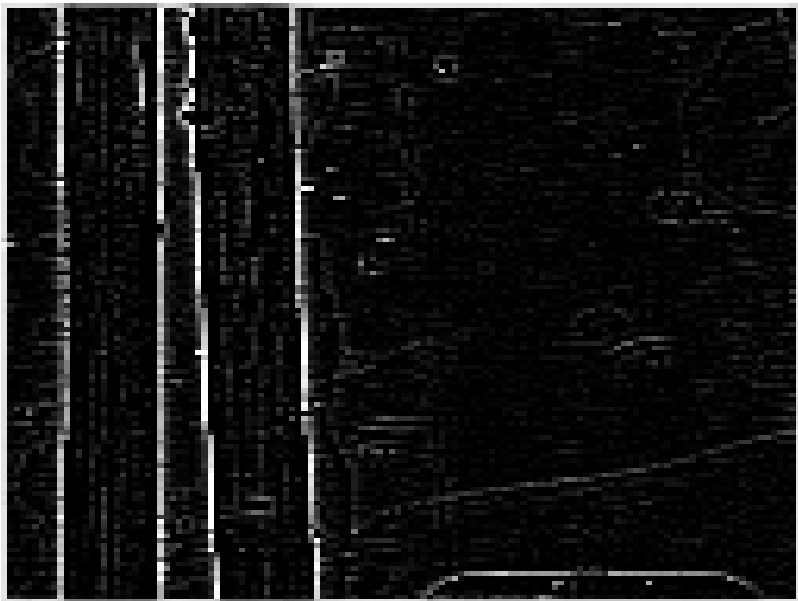

**User:**

Based on your analysis and the tools used, please provide your final classification regarding the presence of eelgrass wasting disease in the image. Provide a brief explanation for your decision, including key observations and any tool results that influenced your conclusion. Consider the color, texture, and pattern of the eelgrass leaves, as well as any visible lesions or discoloration that might indicate disease. At the end of your response, you must provide your classification in the following format: [Yes:PercentYes,No:PercentNo], where PercentYes is the probability you think eelgrass wasting disease is present, and PercentNo is the probability you think it is not present. These percentages must sum to 100%. To break ties, always assign at least 51% to one category. For example, [Yes:75,No:25] indicates 75% certainty of eelgrass wasting disease presence, while [Yes:49,No:51] indicates 51% certainty of its absence.

**Assistant:**

Based on the analysis and the tools used, here is the final classification regarding the presence of eelgrass wasting disease in the image:

**Key Observations:**

- Initial Visual Inspection:** The initial inspection showed a dark streak on the left blade, which could be an early sign of eelgrass wasting disease.
- IncreaseContrastTool:** Enhanced the visibility of the dark streak, making it more prominent but did not reveal additional significant lesions or blotches.
- SharpenTool:** Further enhanced the edges and details, confirming the presence of the dark streak but still no extensive blotching or leaf thinning.
- PredictEelgrassWastingDiseaseTool:** The machine learning model predicted a low probability (7.13%) of eelgrass wasting disease, suggesting that the observed features might not be indicative of the disease.
- EdgeDetectionTool:** Highlighted the boundaries and features, showing the dark streak more clearly but did not reveal additional patterns or lesions typical of eelgrass wasting disease.

**Conclusion:**

The combination of visual inspection and tool results suggests that while there is a dark streak present, it does not exhibit the extensive symptoms typically associated with eelgrass wasting disease, such as large blotches, significant leaf thinning, or widespread dieback. The low probability from the PredictEelgrassWastingDiseaseTool further supports this conclusion.

Therefore, I classify the image as not showing eelgrass wasting disease.

[Yes:20,No:80]
