# Supplementary material for: AiSciVision: A Framework for Specializing Large Multimodal Models in Scientific Image Classification
Source: arXiv:2410.21480 source file (2024-10-28)
Supplement: Supplementary file 6 [file visrag_true1_lmm1_sup0.pdf]

True Class: 1, LMM Prediction: 1 (Probability: 0.85), Supervised Prediction: 0 (Probability: 7.13)

**System:**

You are an expert marine biologist specializing in eelgrass wasting disease classification. Your task is to determine whether an scan of an eelgrass blade contains eelgrass wasting disease or not. Eelgrass wasting disease, primarily caused by the marine pathogen *Labyrinthula zosterae*, presents visually as dark, necrotic lesions on the leaves of eelgrass (*Zostera marina*). These lesions typically appear as irregular black or brown spots or streaks, often starting at the tips of the leaves and spreading downwards. Over time, these lesions can coalesce, leading to extensive damage, including:

1. Spotting and Streaking: Initial symptoms include small, dark spots or streaks on the eelgrass leaves.
2. Blotching: As the disease progresses, these spots merge into larger blotches, which may appear dark brown or black.
3. Leaf Thinning and Loss: Affected areas may thin out or deteriorate, causing leaves to become more fragile and eventually break off.
4. Overall Decline: Heavily infected eelgrass beds often exhibit widespread dieback, with leaves appearing discolored, tattered, or decomposed.

Use your knowledge and the tools provided to make an accurate classification.

**User:**

I will start by first showing you an example image, that is visually similar to the image we want to classify, that does have eelgrass wasting disease. Then I will show you another example image that does not have eelgrass wasting disease, but is visually similar to the image we want to classify. Then I will show you the image we want to classify. For the first two, you should briefly (1-2 sentences) explain why it does or does not have eelgrass wasting disease. For the final image you should explain in a paragraph why you believe it does or does not have eelgrass wasting disease.

Here is the example that does have eelgrass wasting disease, only respond describing it, nothing else:

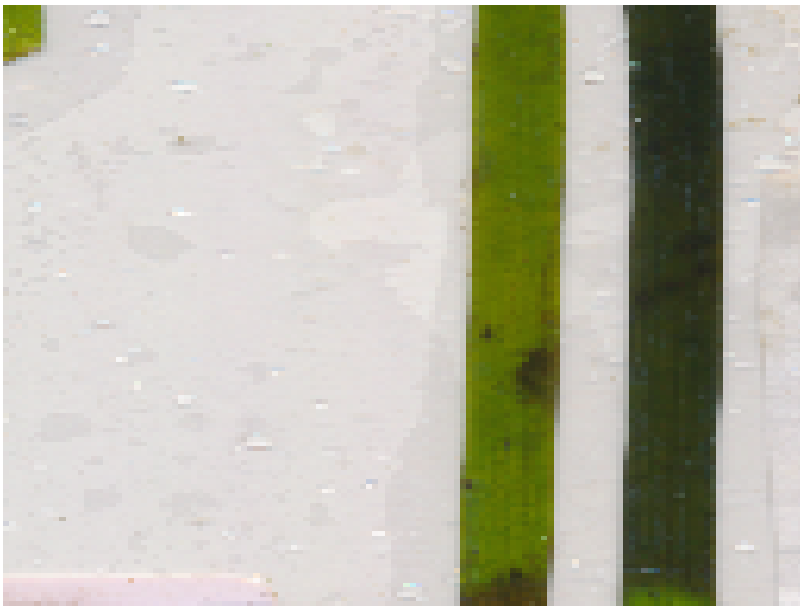

**Assistant:**

This image shows eelgrass blades with dark, necrotic lesions, which are indicative of eelgrass wasting disease. The dark spots and streaks on the leaves are characteristic symptoms of the disease.

**User:**

Here is the example that does not have eelgrass wasting disease only respond describing it, nothing else:

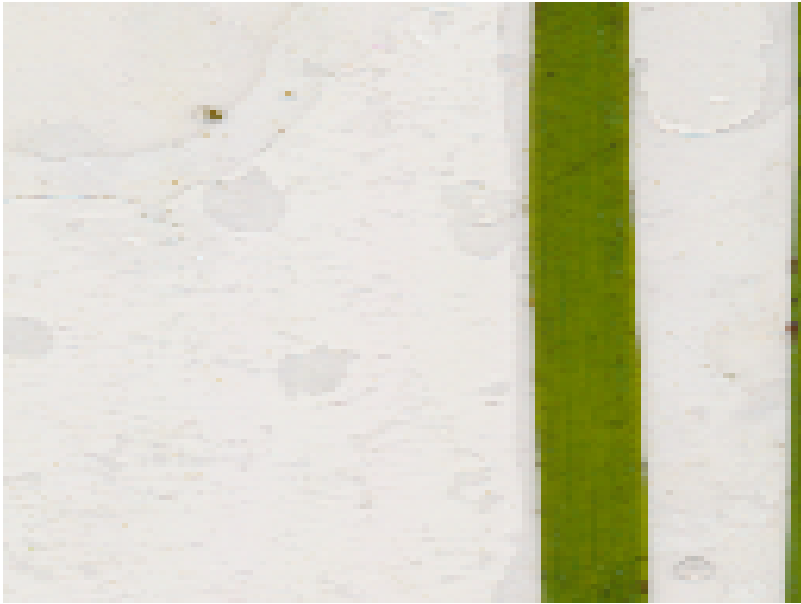

**Assistant:**

This image shows eelgrass blades that appear healthy, with no visible dark spots, streaks, or necrotic lesions. The leaves are uniformly green and free from any signs of eelgrass wasting disease.

**User:**

Here is the image need to classify as having eelgrass wasting disease or not. Describe what you see and compare and contrast it with the previous two known examples. Explain your thought process for classifying this image.

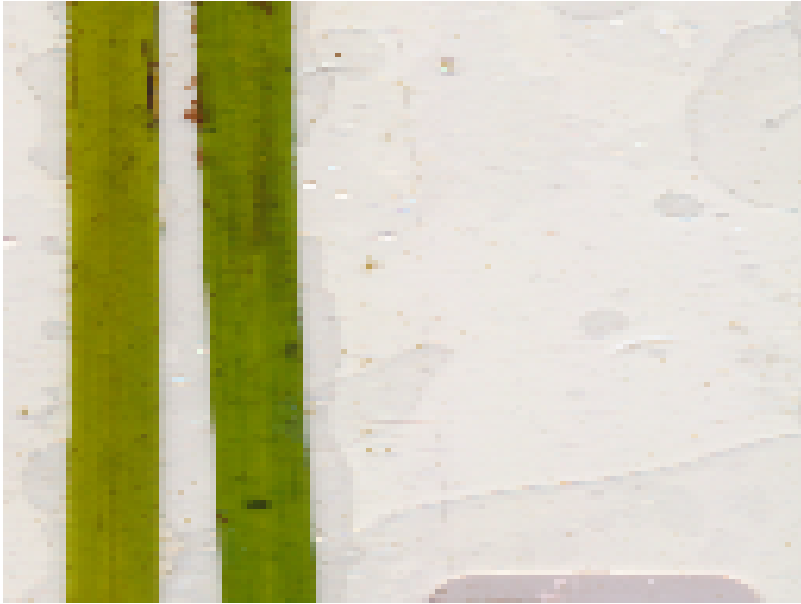

**Assistant:**

In this image, the eelgrass blades exhibit some dark spots and streaks, particularly on the left blade. These dark areas are similar to the necrotic lesions seen in the first example image, which had eelgrass wasting disease. The presence of these dark spots and streaks contrasts with the uniformly green and healthy appearance of the eelgrass blades in the second example image, which did not have the disease.

Comparing this image to the first example, the dark spots and streaks are indicative of the initial symptoms of eelgrass wasting disease. Although the lesions are not as extensive as in the first example, their presence suggests the onset of the disease. Therefore, based on the visual evidence of dark, necrotic lesions, I classify this image as showing eelgrass wasting disease.

### User:

Based on your analysis and the tools used, please provide your final classification regarding the presence of eelgrass wasting disease in the image. Provide a brief explanation for your decision, including key observations and any tool results that influenced your conclusion. Consider the color, texture, and pattern of the eelgrass leaves, as well as any visible lesions or discoloration that might indicate disease. At the end of your response, you must provide your classification in the following format:

[Yes:PercentYes,No:PercentNo], where PercentYes is the probability you think eelgrass wasting disease is present, and PercentNo is the probability you think it is not present. These percentages must sum to 100%. To break ties, always assign at least 51% to one category. For example, [Yes:75,No:25] indicates 75% certainty of eelgrass wasting disease presence, while [Yes:49,No:51] indicates 51% certainty of its absence.

### Assistant:

Based on the analysis of the image, the eelgrass blades exhibit dark spots and streaks, particularly on the left blade. These dark areas are consistent with the initial symptoms of eelgrass wasting disease, which include necrotic lesions that appear as irregular black or brown spots or streaks. The presence of these lesions, even though not as extensive as in the first example, suggests the onset of the disease.

Key observations include: - Dark spots and streaks on the left blade, which are indicative of necrotic lesions. - The pattern and texture of these lesions are similar to those seen in the first example image with eelgrass wasting disease. - The overall appearance of the eelgrass blades shows signs of discoloration and potential disease onset.

Considering these observations and the comparison with the known examples, I conclude that there is a high probability that eelgrass wasting disease is present in this image.

Final classification: [Yes:85,No:15]
